# Supplementary material for: Audio-Guided Visual Editing with Complex Multi-Modal Prompts
Source: arXiv:2508.20379 source file (2025-08-28)
Supplement: Supplementary file 1 [file figure_TA2I_supp.pdf]

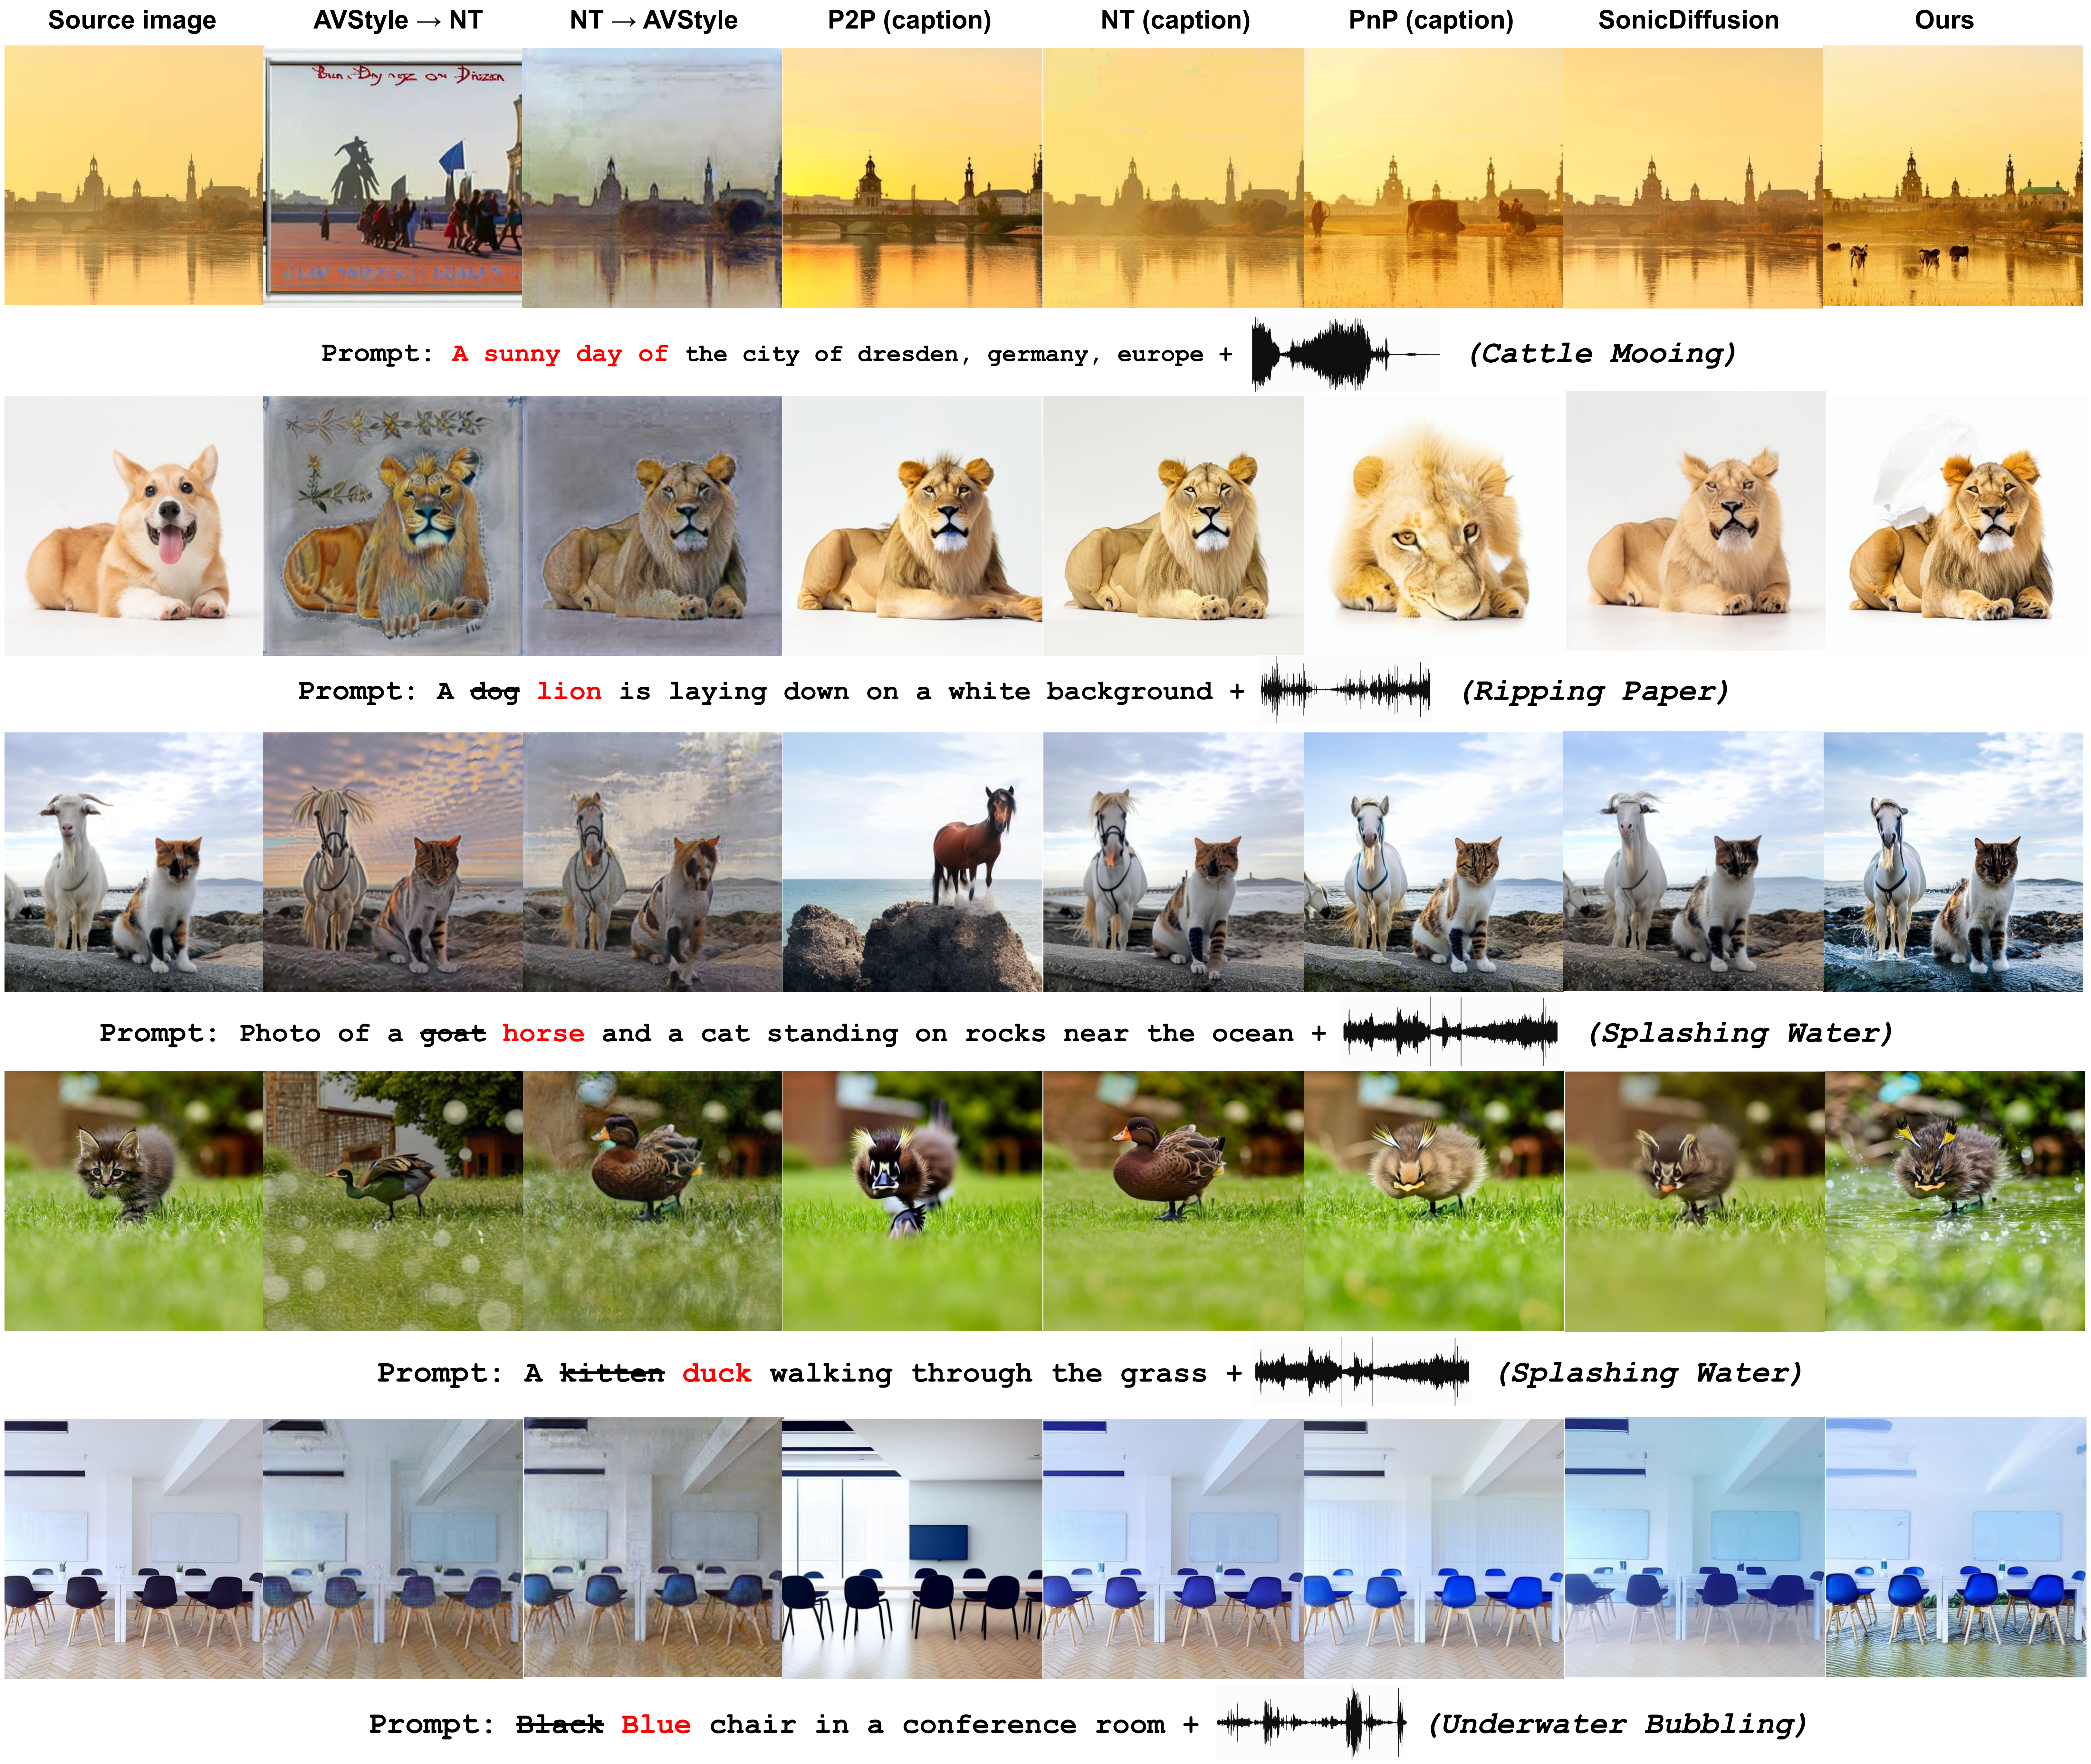
Source image
AVStyle → NT
NT → AVStyle
P2P (caption)
NT (caption)
PnP (caption)
SonicDiffusion
Ours
Prompt: A sunny day of the city of dresden, germany, europe +
(Cattle Mooing)
Prompt: A ~~dog~~ lion is laying down on a white background +
(Ripping Paper)
Prompt: Photo of a ~~goat~~ horse and a cat standing on rocks near the ocean +
(Splashing Water)
Prompt: A ~~kitten~~ duck walking through the grass +
(Splashing Water)
Prompt: ~~Black~~ Blue chair in a conference room +
(Underwater Bubbling)

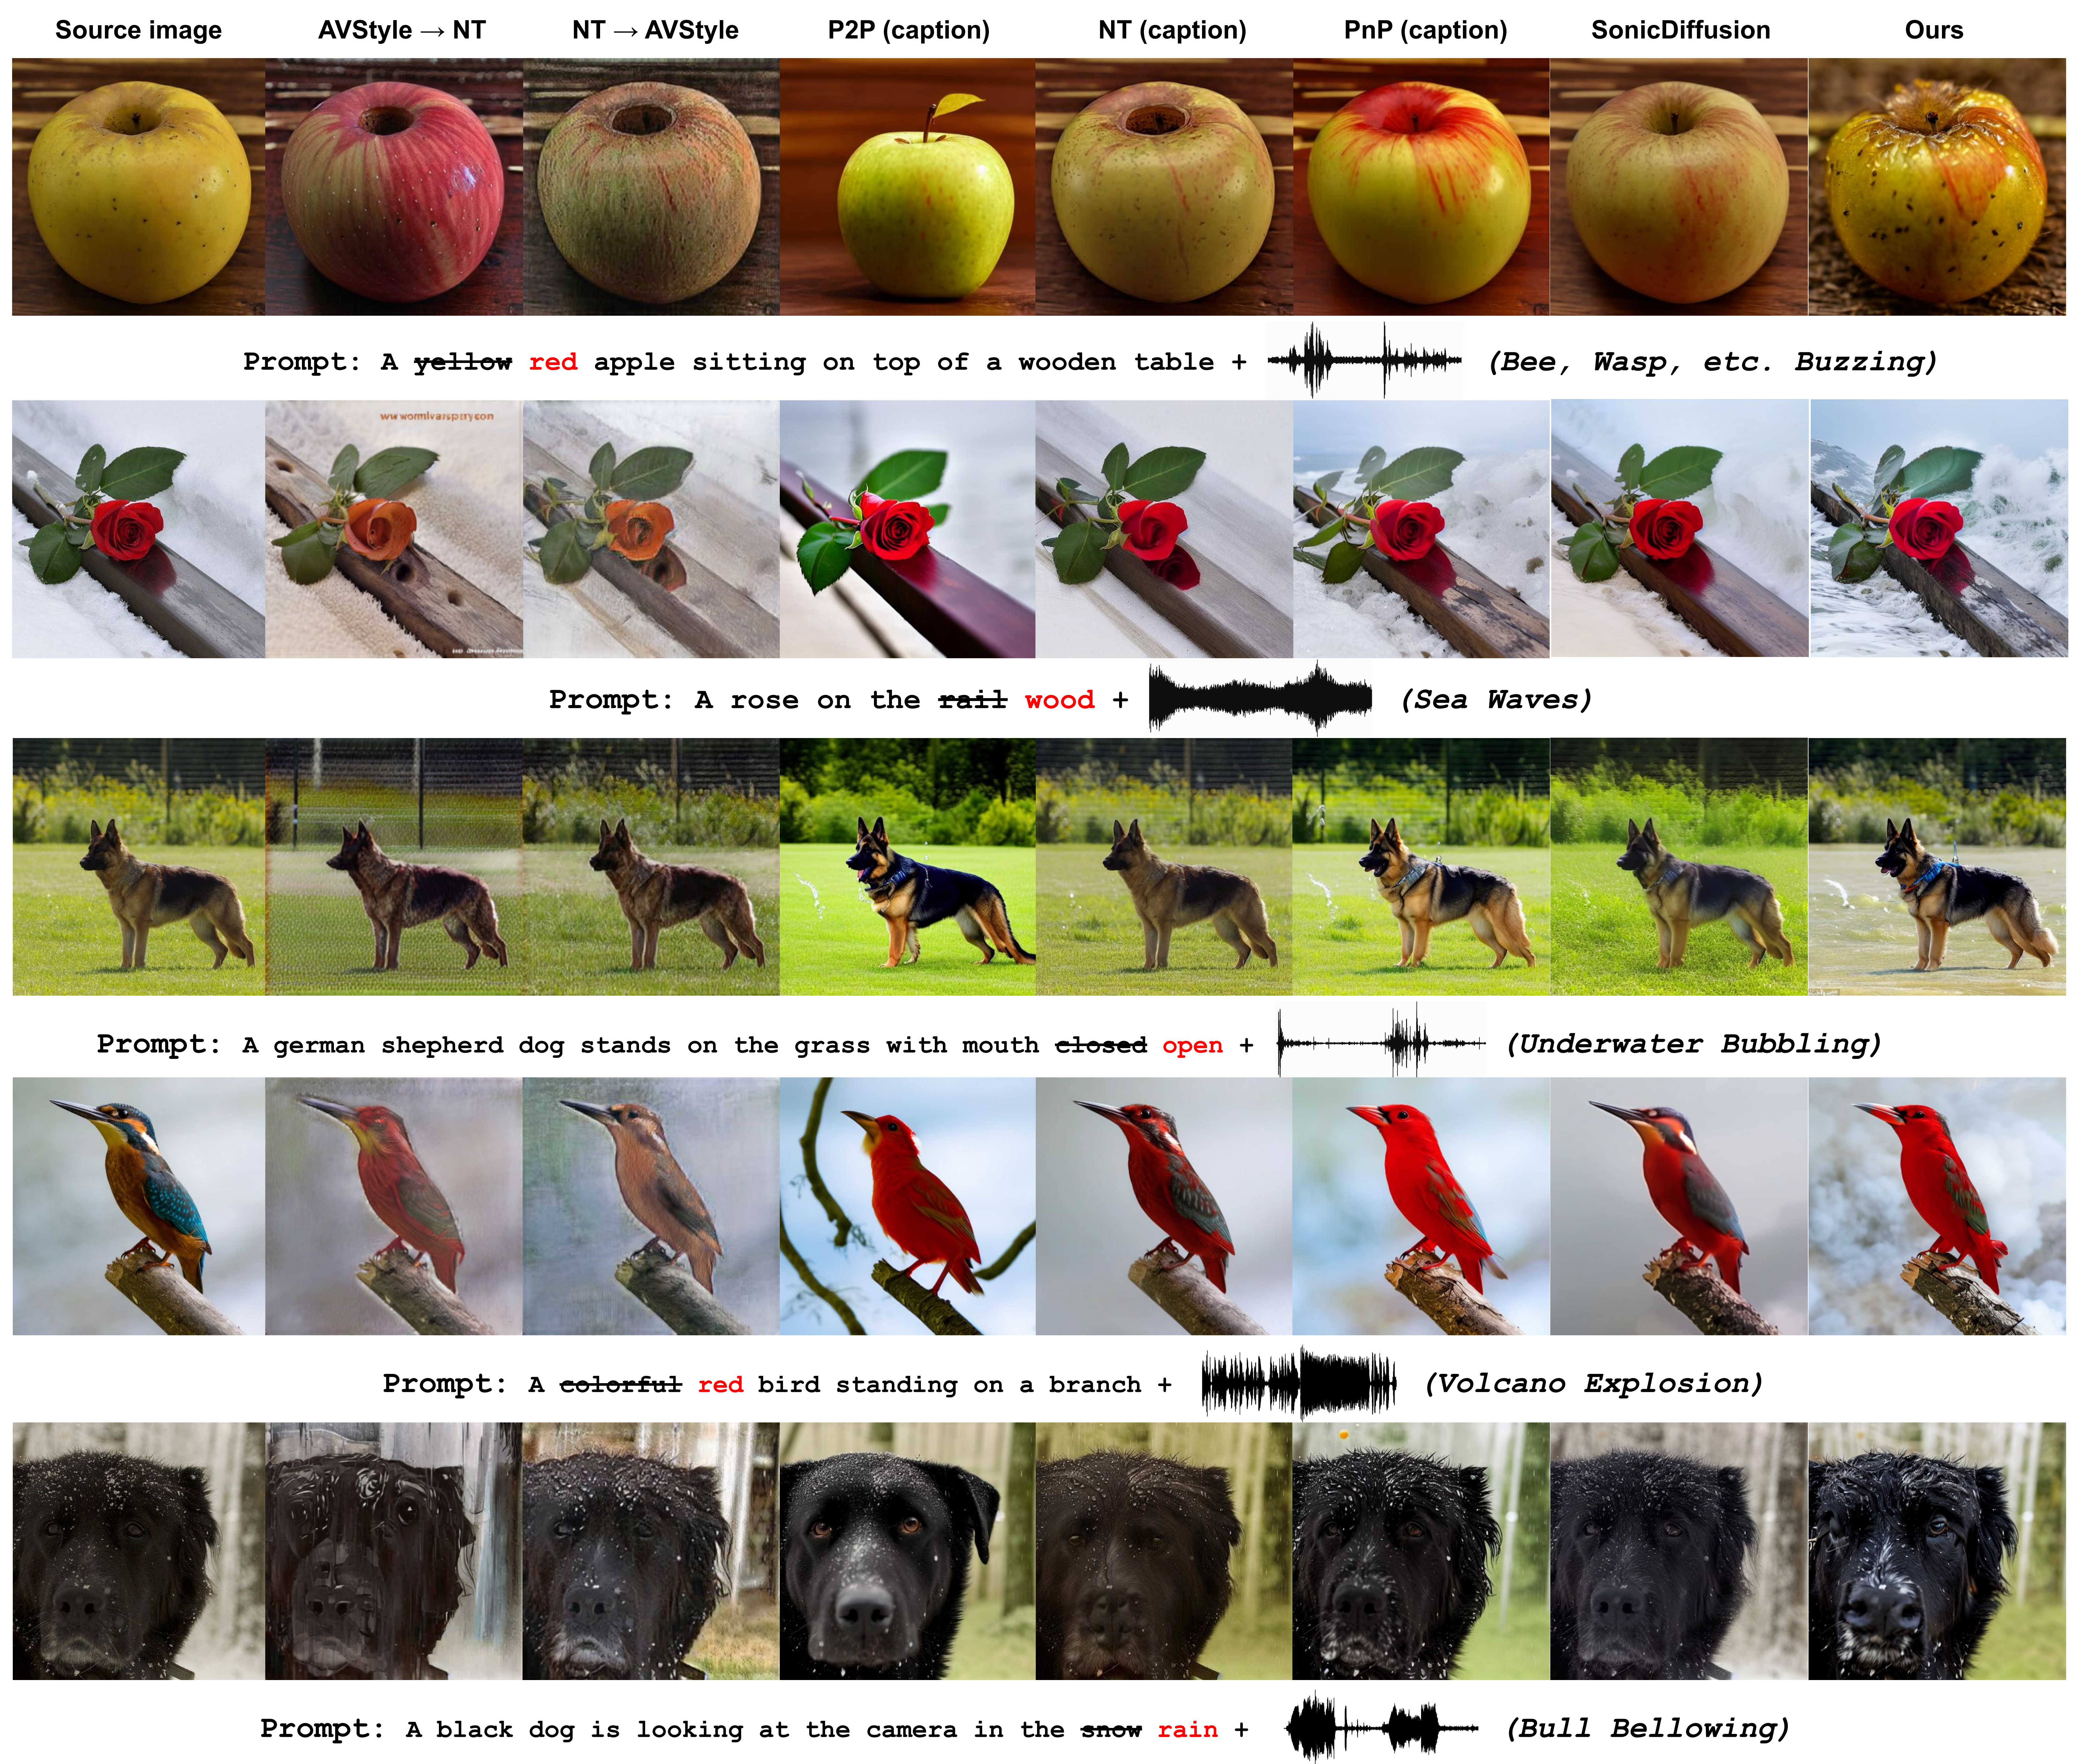
Source image
AVStyle → NT
NT → AVStyle
P2P (caption)
NT (caption)
PnP (caption)
SonicDiffusion
Ours
Prompt: A ~~yellow~~ red apple sitting on top of a wooden table + (Bee, Wasp, etc. Buzzing)
Prompt: A rose on the ~~rail~~ wood + (Sea Waves)
Prompt: A german shepherd dog stands on the grass with mouth ~~closed~~ open + (Underwater Bubbling)
Prompt: A ~~colorful~~ red bird standing on a branch + (Volcano Explosion)
Prompt: A black dog is looking at the camera in the ~~snow~~ rain + (Bull Bellowing)
