# Supplementary material for: Audio-Guided Visual Editing with Complex Multi-Modal Prompts
Source: arXiv:2508.20379 source file (2025-08-28)
Supplement: Supplementary file 2 [file figure_A2I_supp.pdf]

Source image

AVStyle

SonicDiffusion

P2P (caption)

NT (caption)

PnP (caption)

Ours

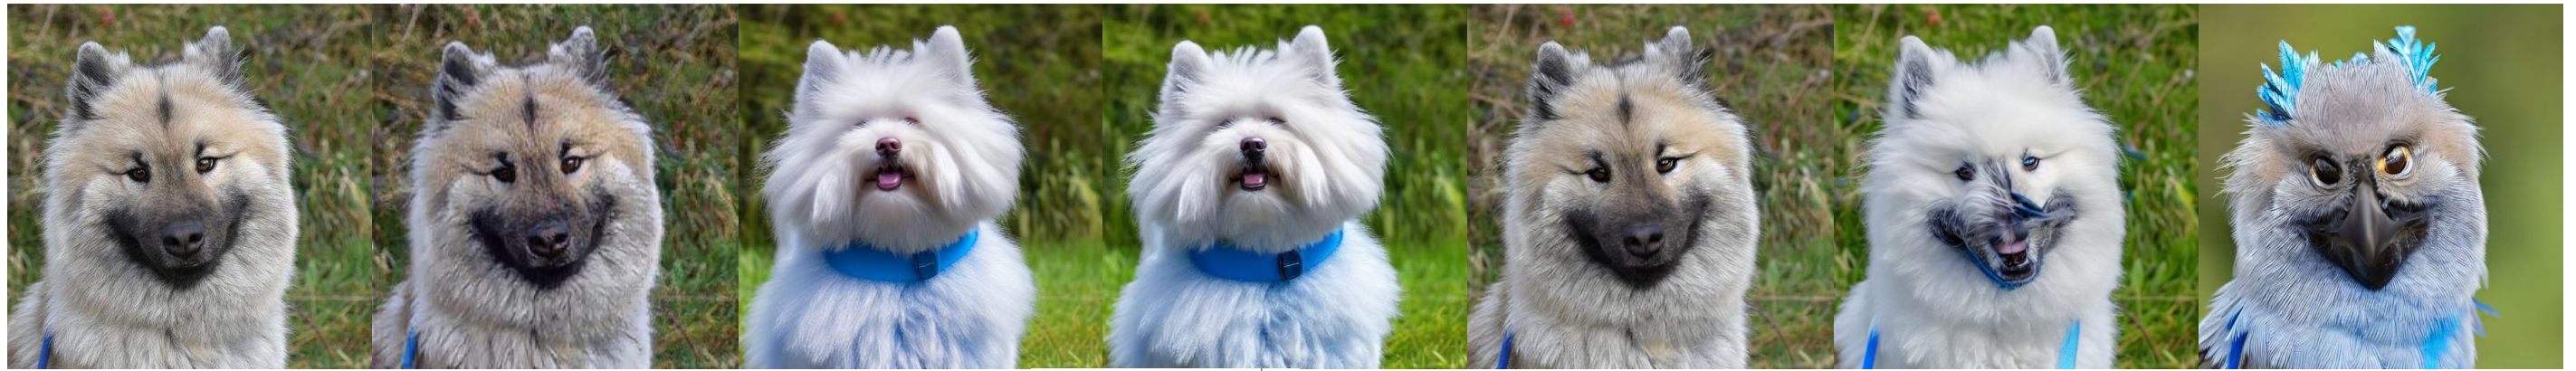

Prompt:

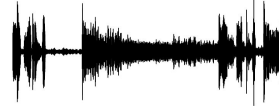*(Bird Chirping, Tweeting)*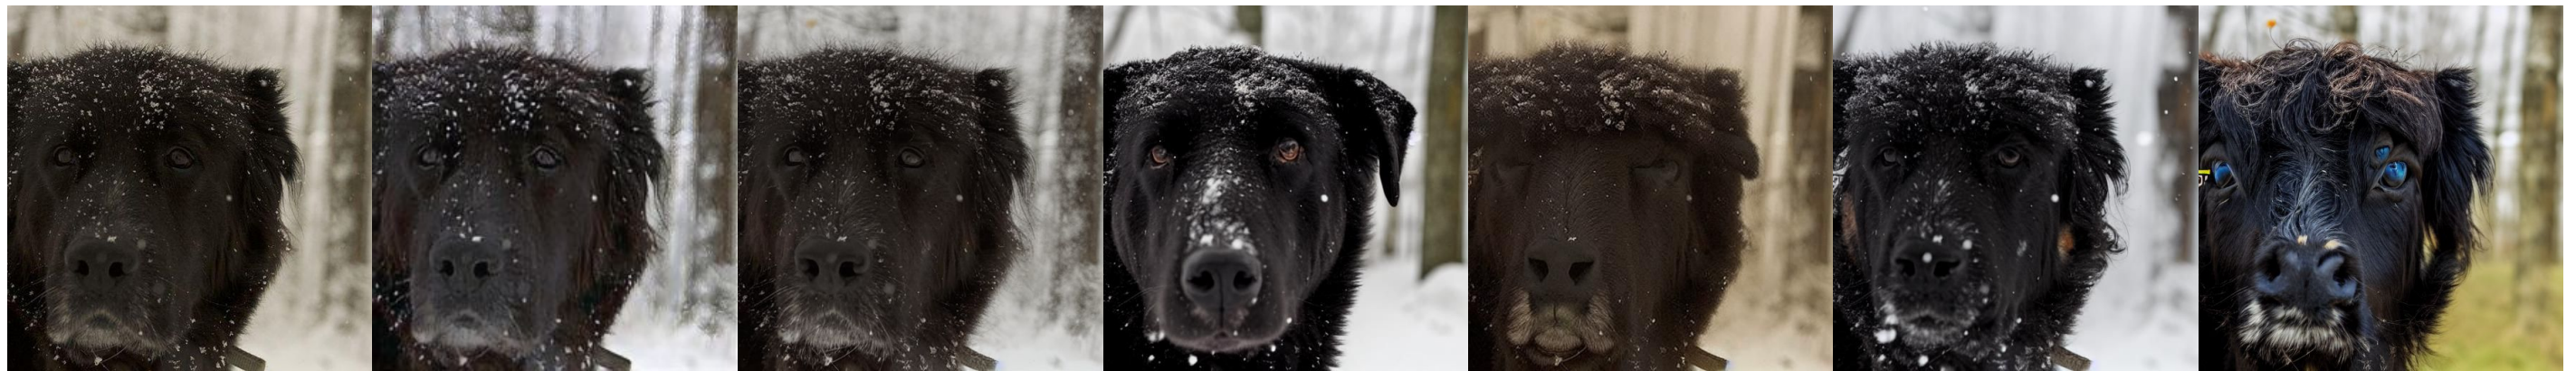

Prompt:

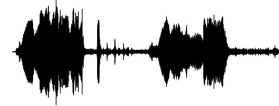*(Bull Bellowing)*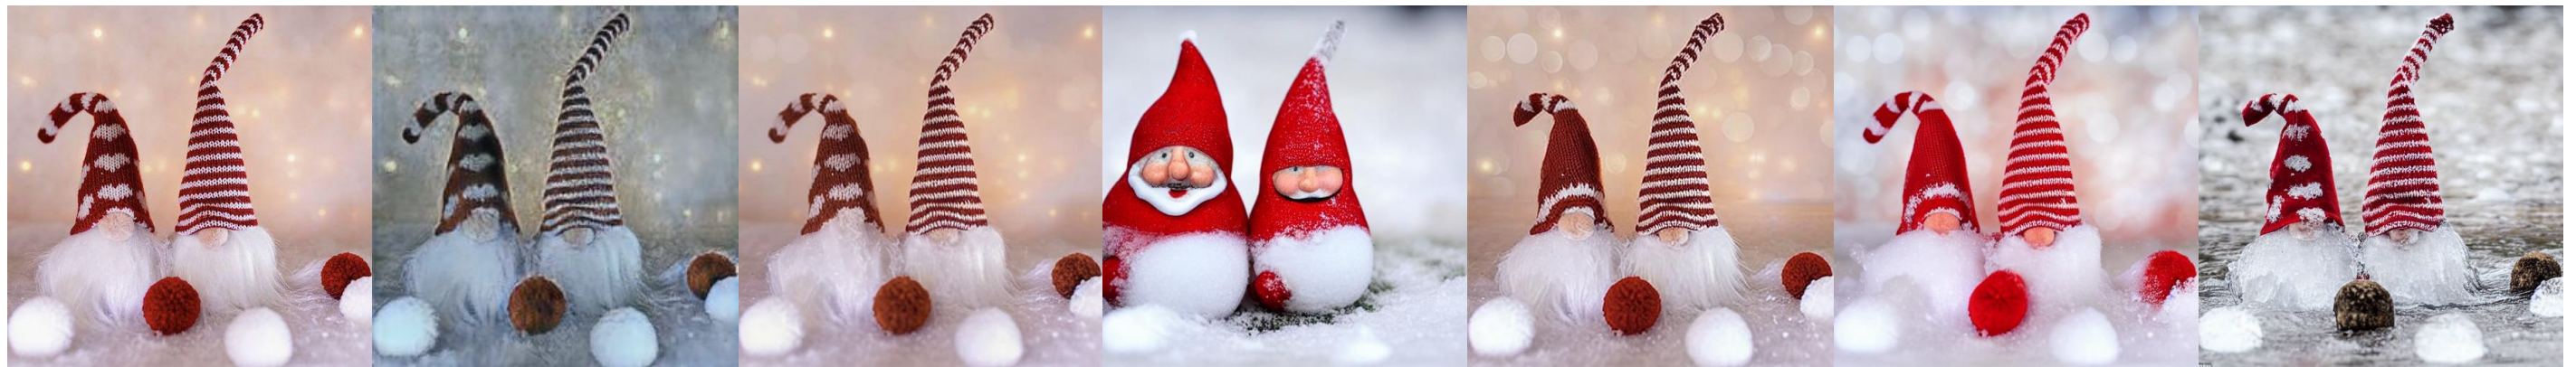

Prompt:

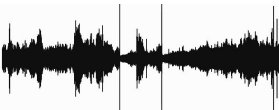*(Splashing Water)*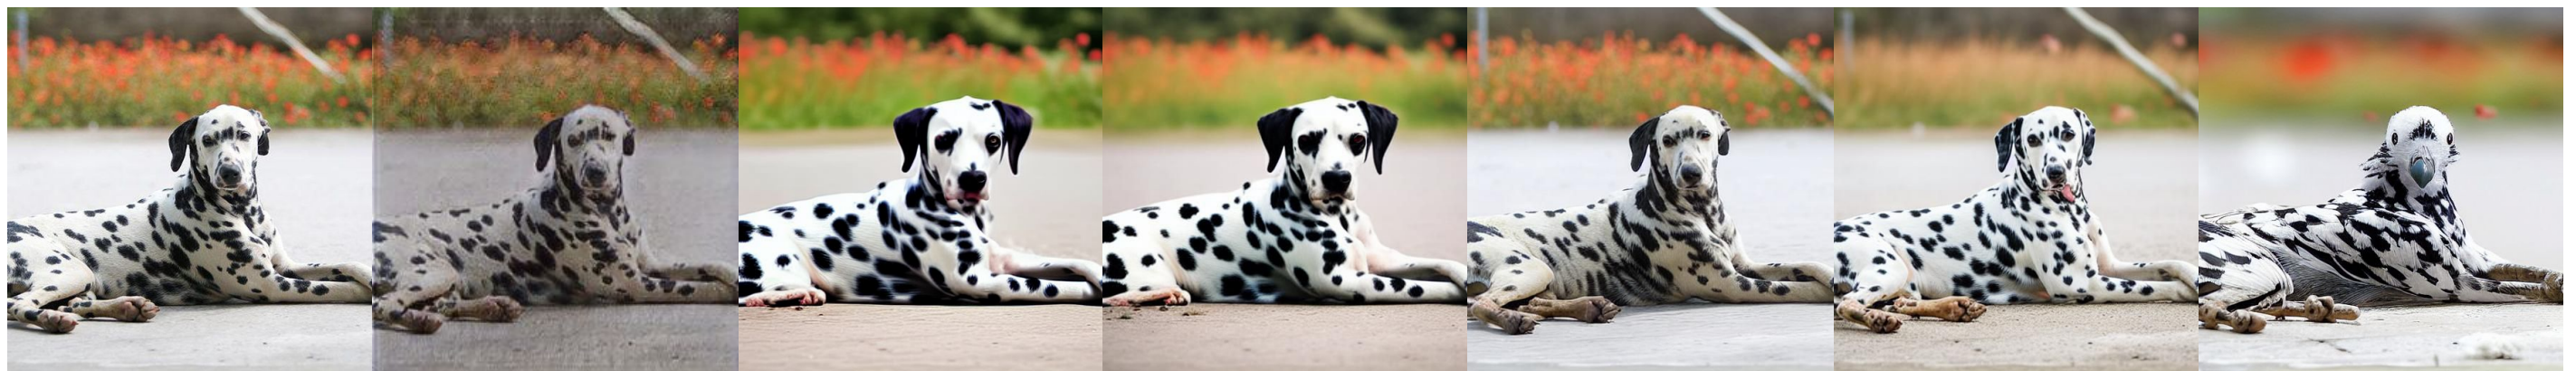

Prompt:

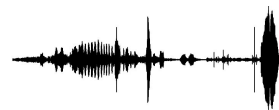*(Bird Squawking)*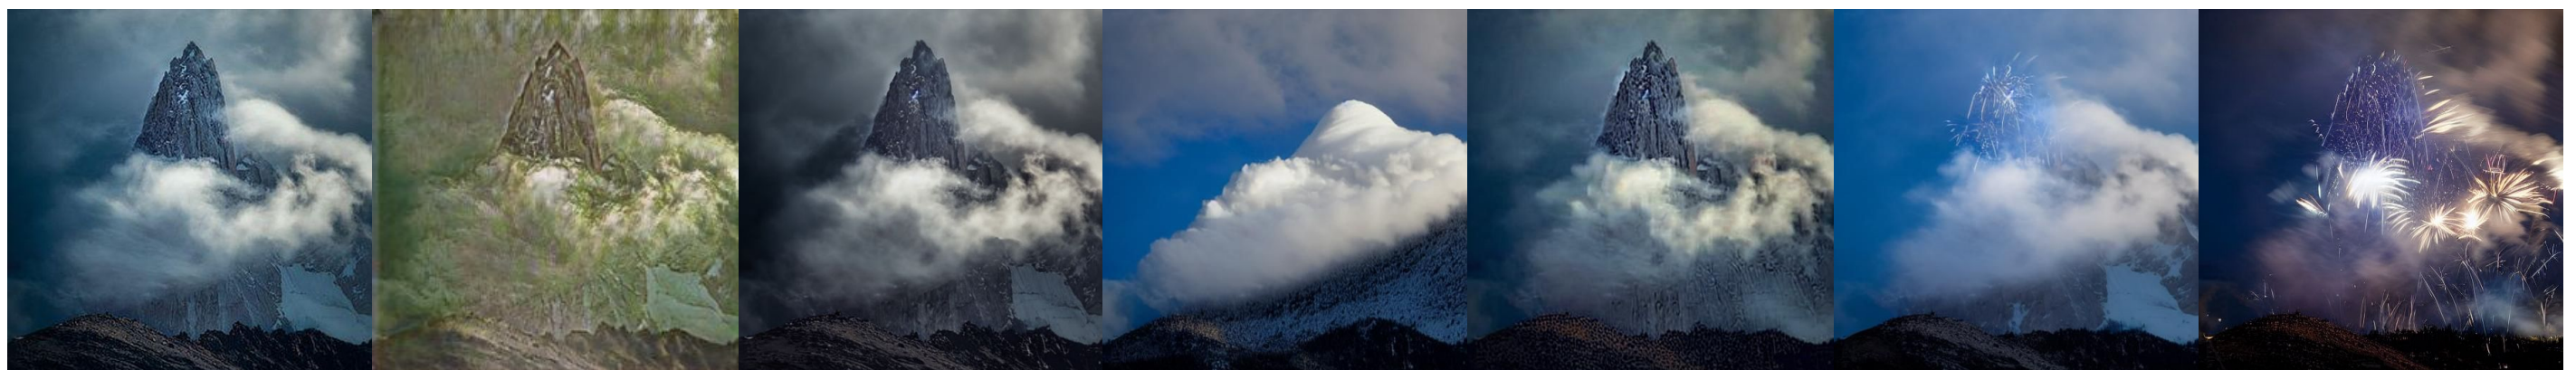

Prompt:

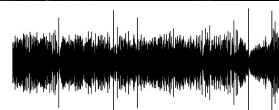*(Fireworks Banging)*



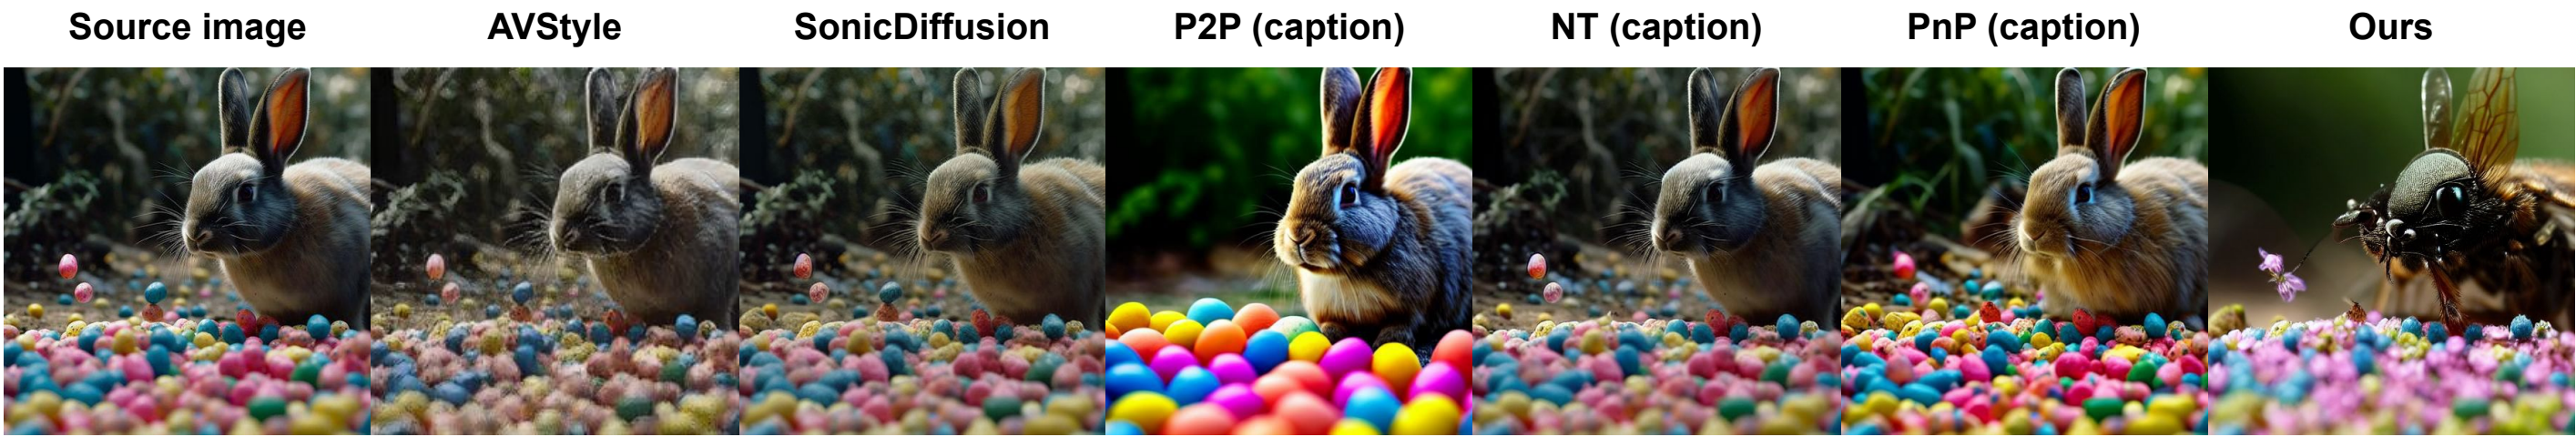

Prompt: 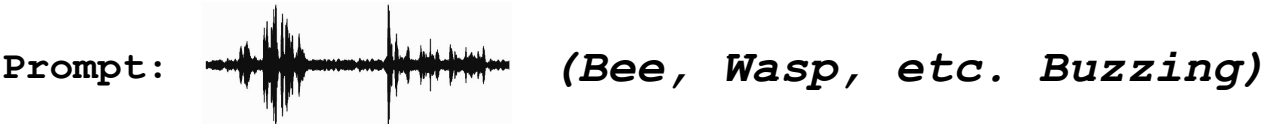 *(Bee, Wasp, etc. Buzzing)*

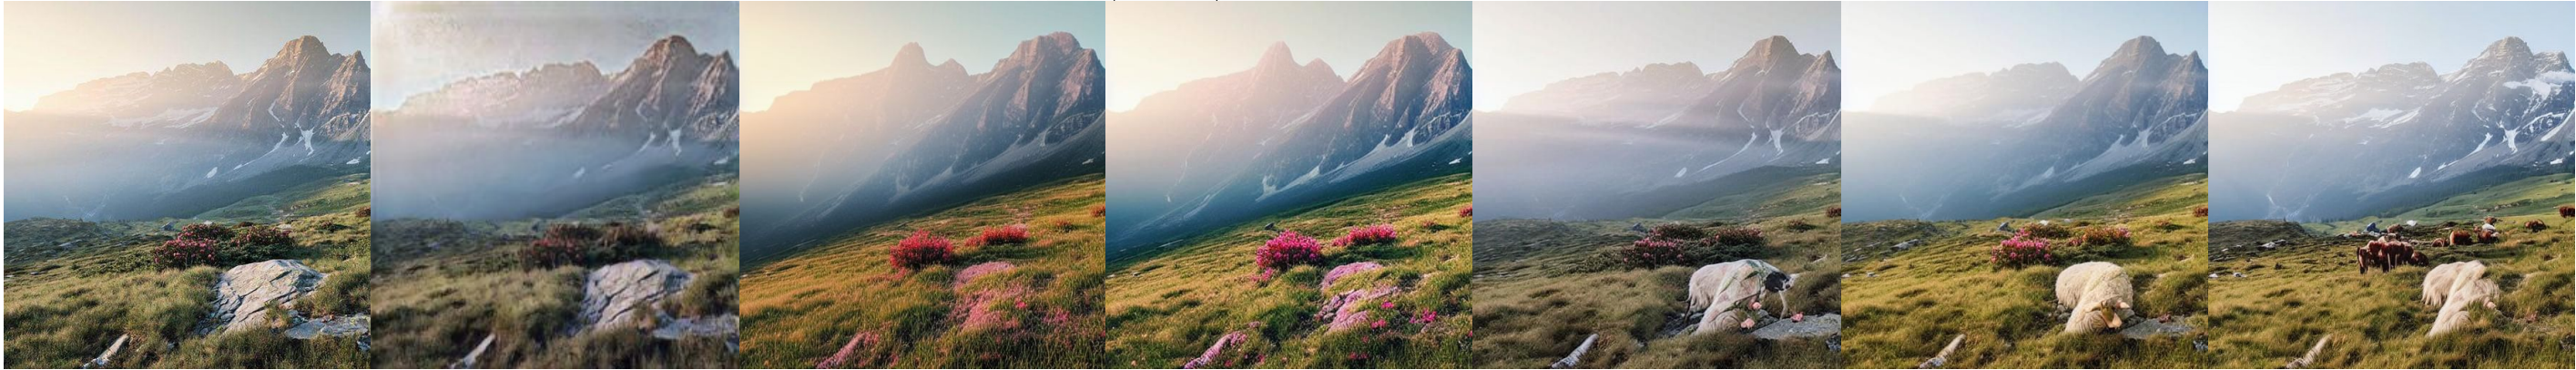

Prompt: 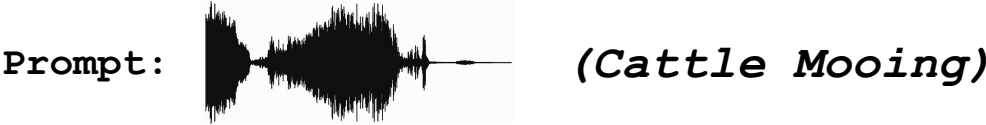 *(Cattle Mooing)*

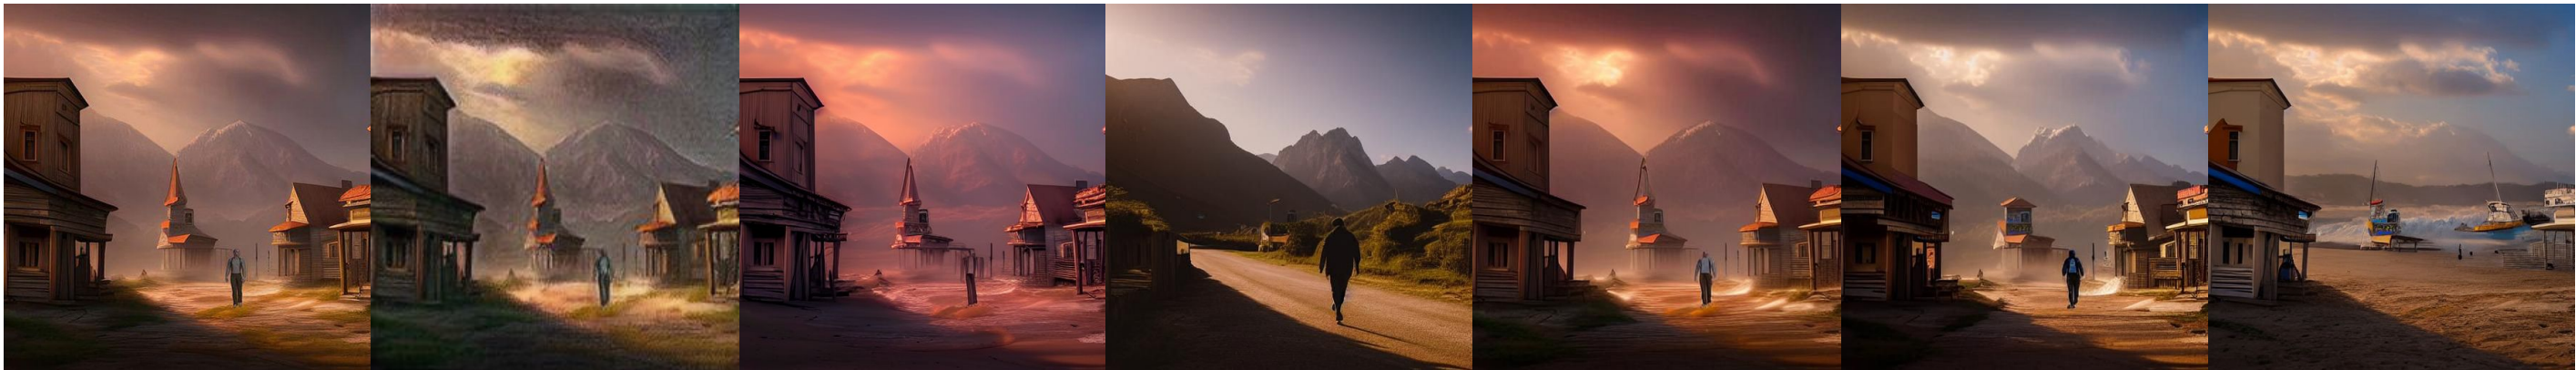

Prompt: 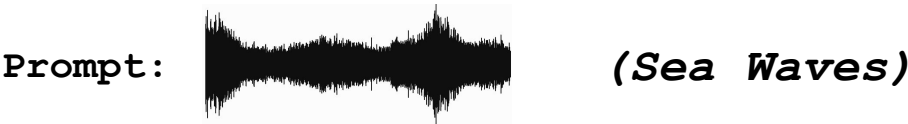 *(Sea Waves)*

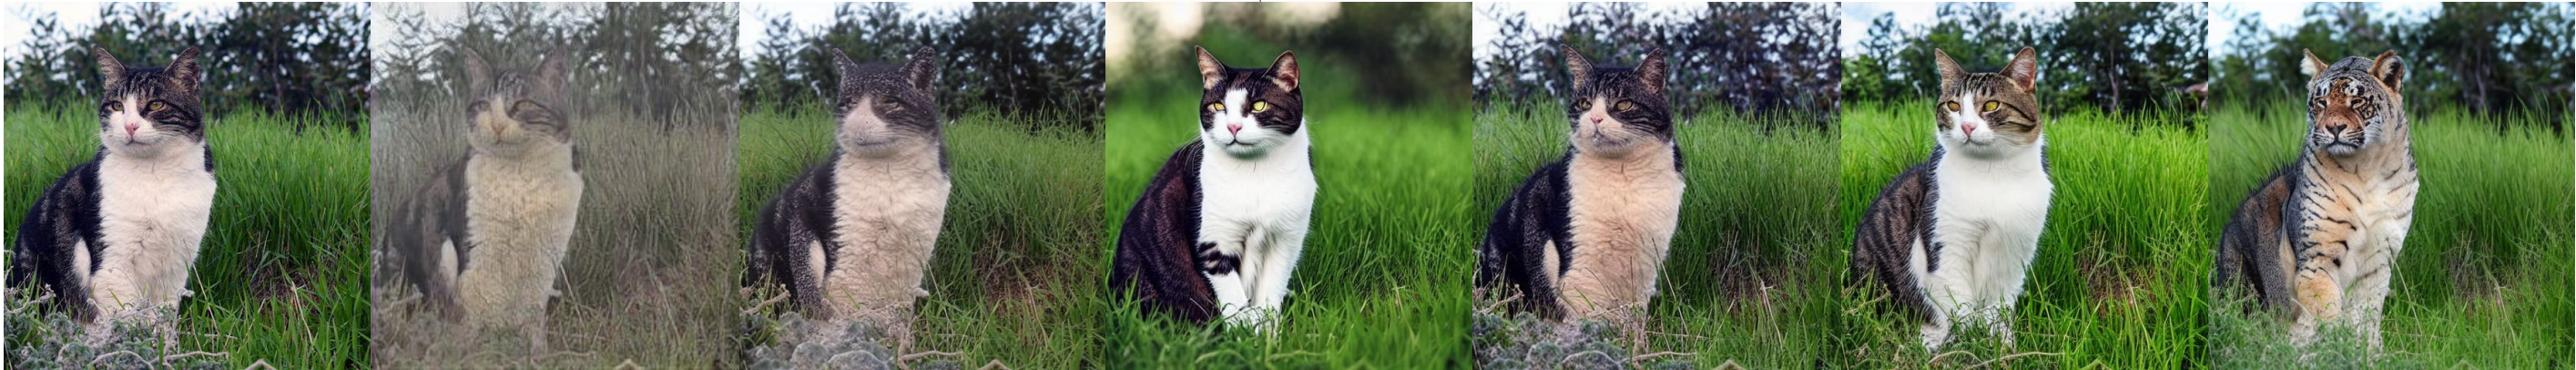

Prompt: 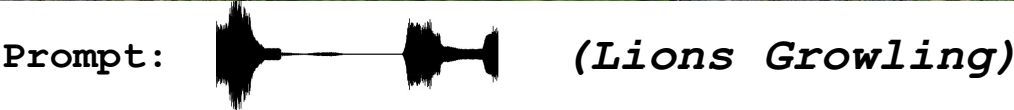 *(Lions Growling)*

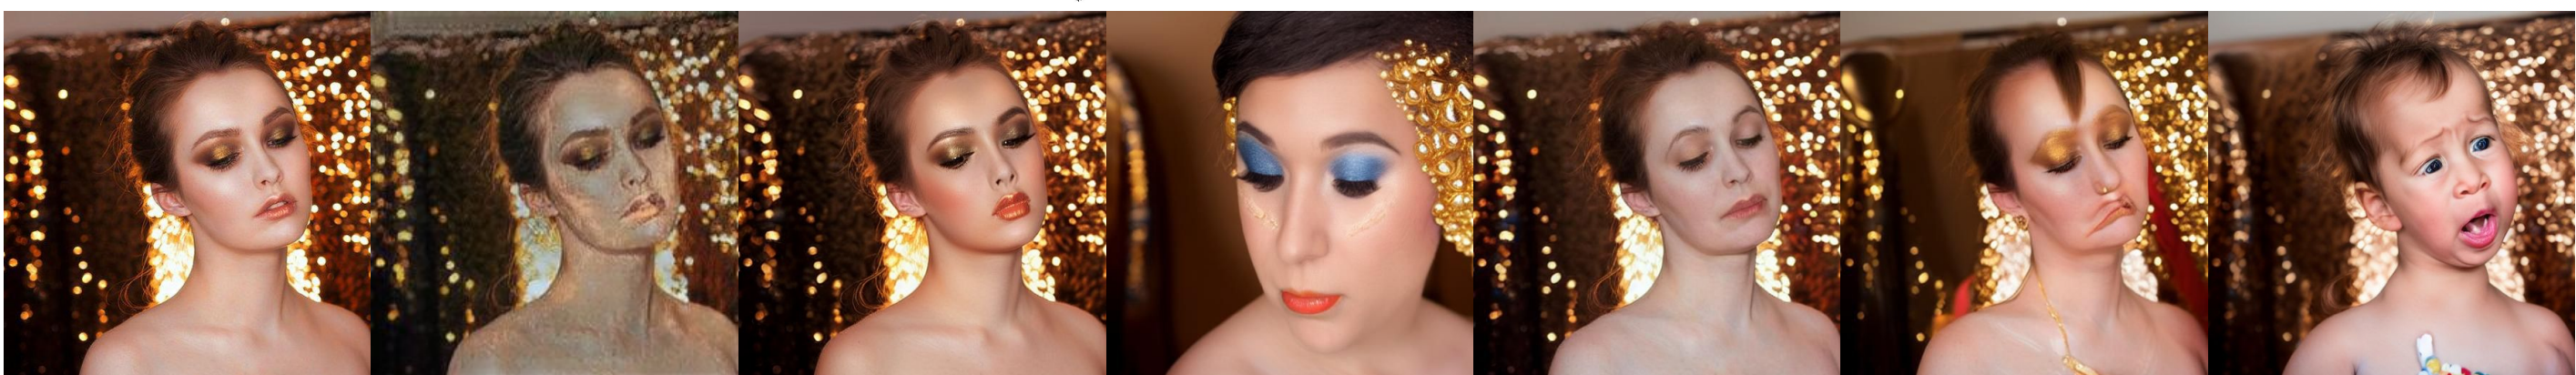

Prompt: 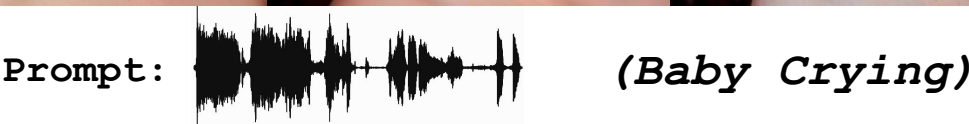 *(Baby Crying)*



Source image

AVStyle

SonicDiffusion

P2P (caption)

NT (caption)

PnP (caption)

Ours

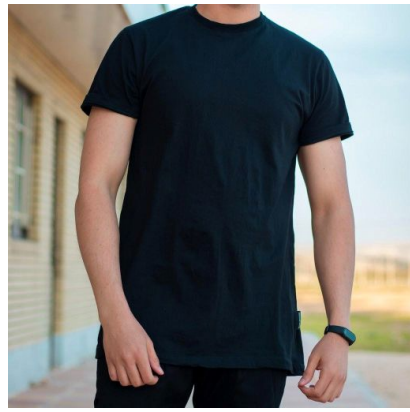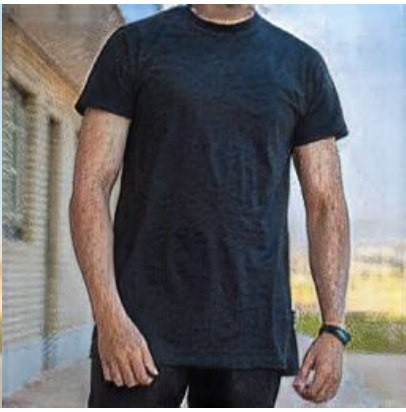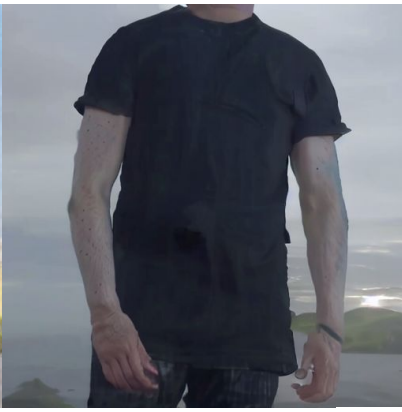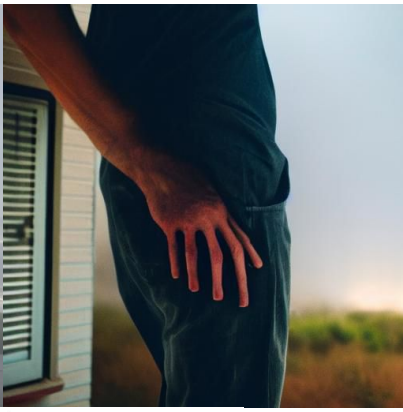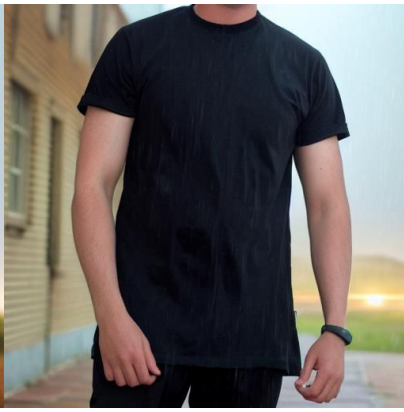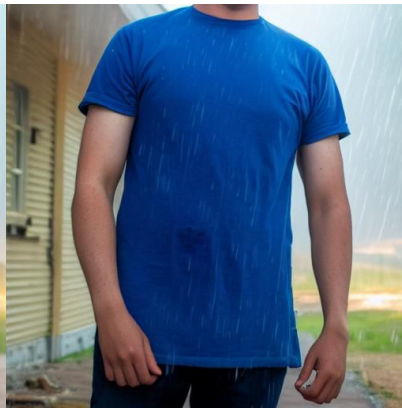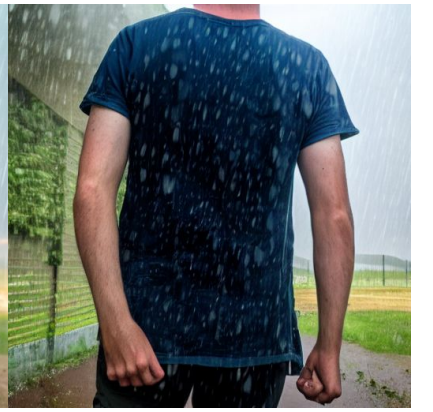

Prompt: 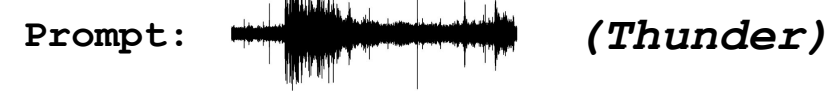 (*Thunder*)

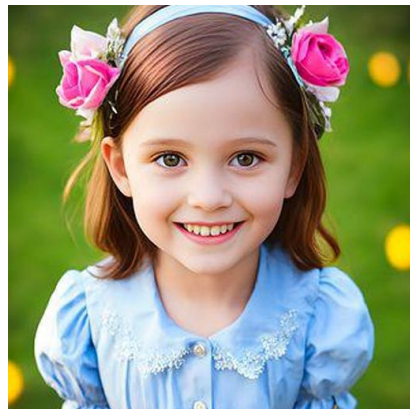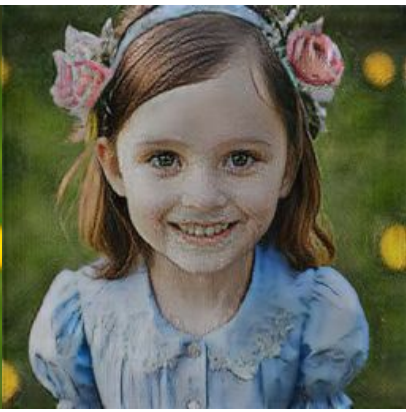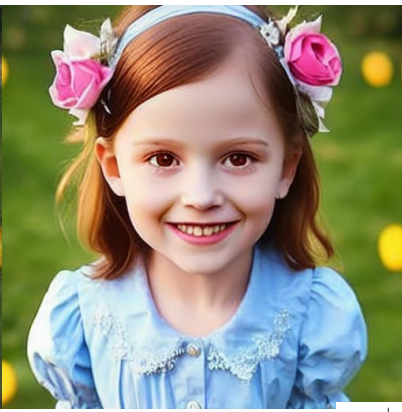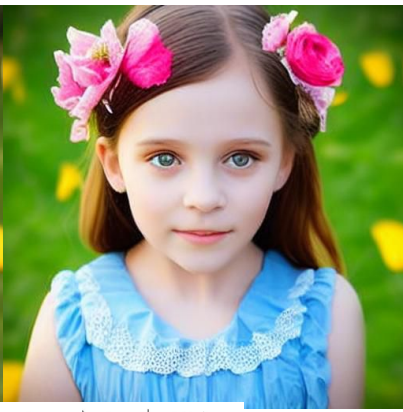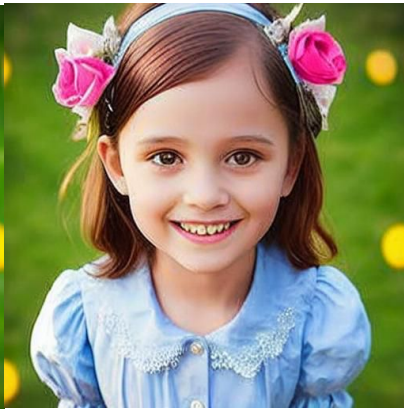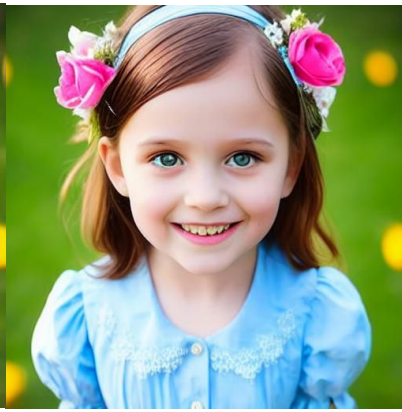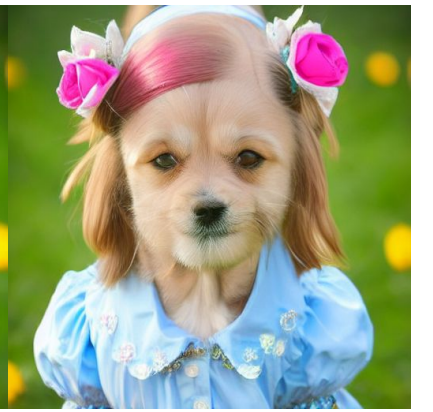

Prompt: 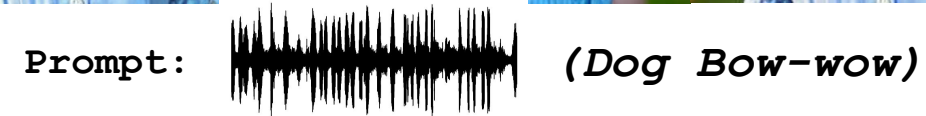 (*Dog Bow-wow*)

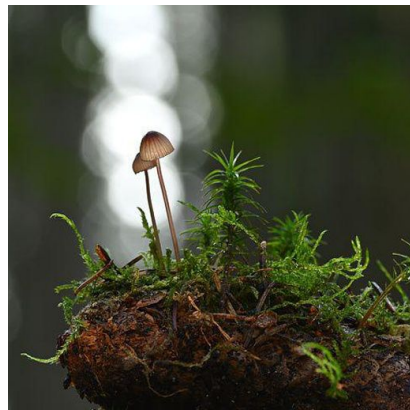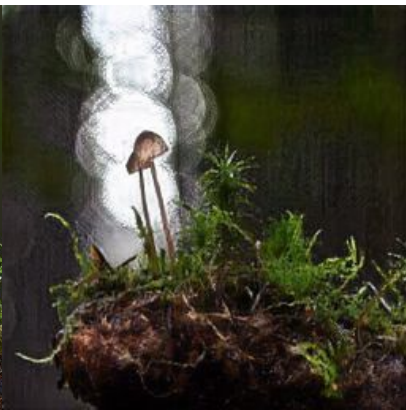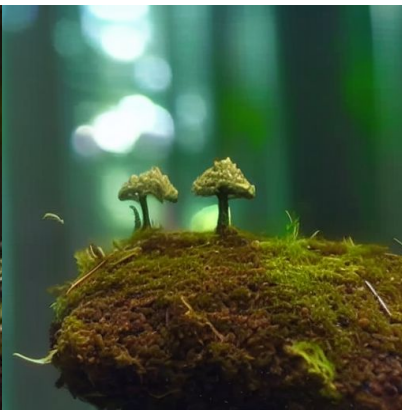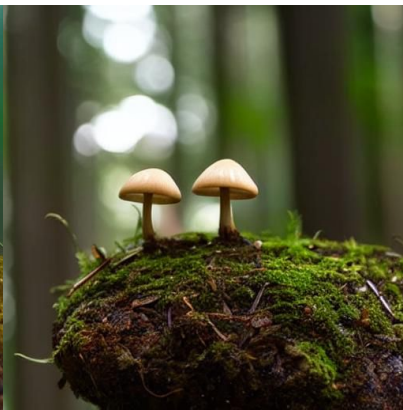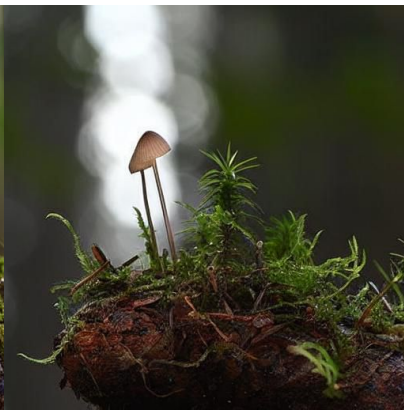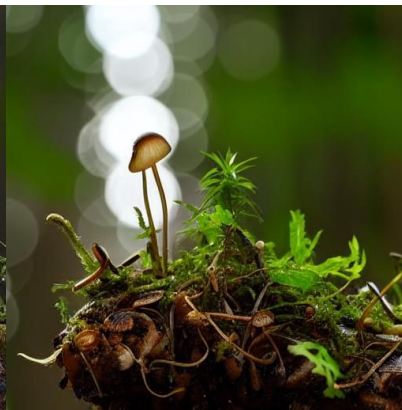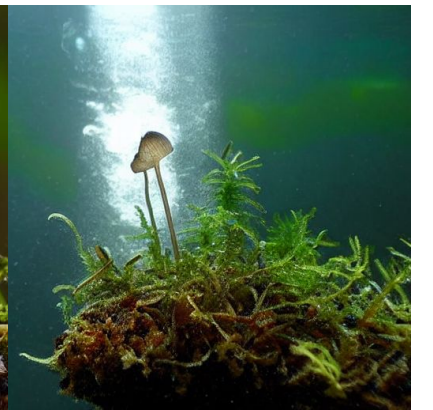

Prompt: 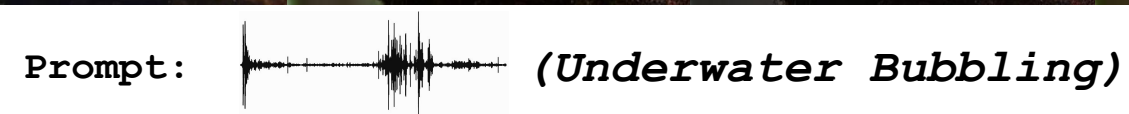 (*Underwater Bubbling*)

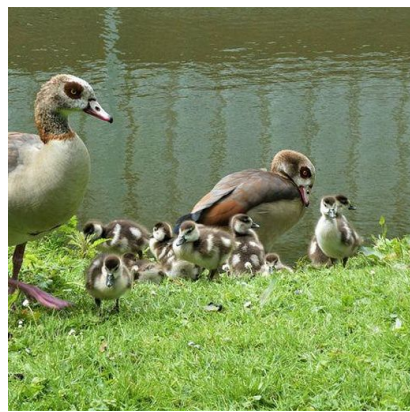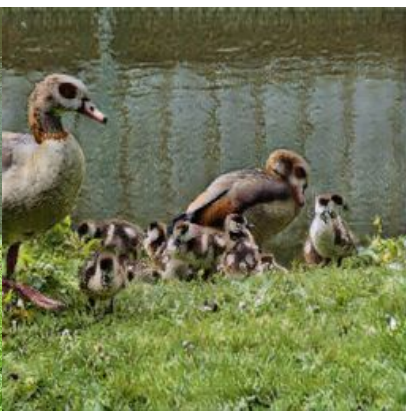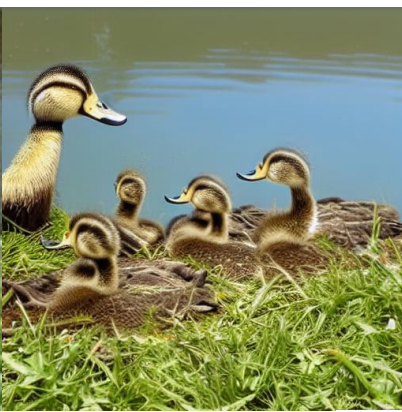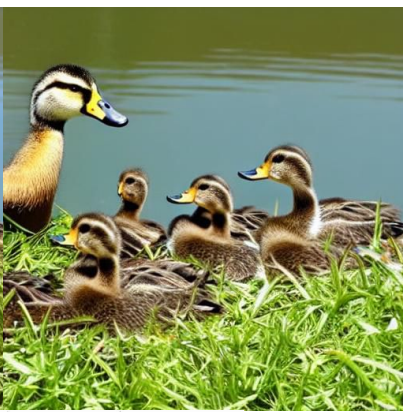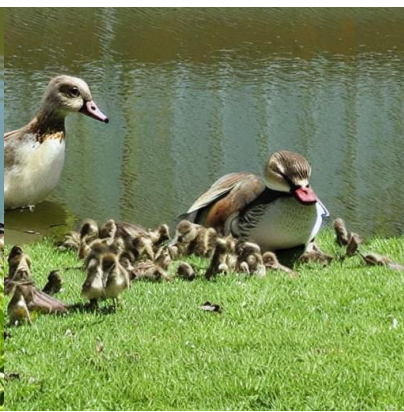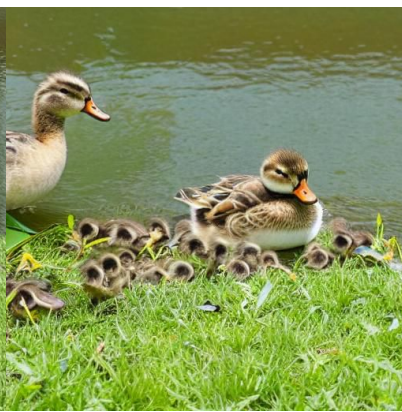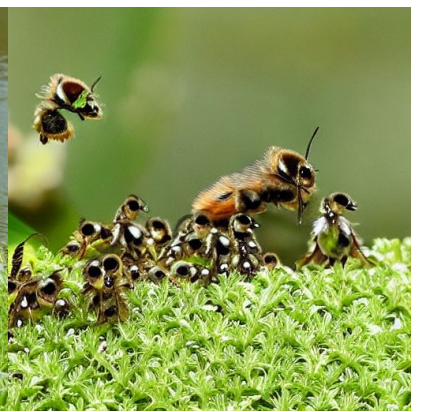

Prompt: 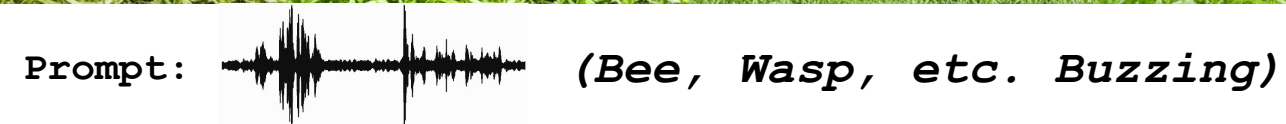 (*Bee, Wasp, etc. Buzzing*)

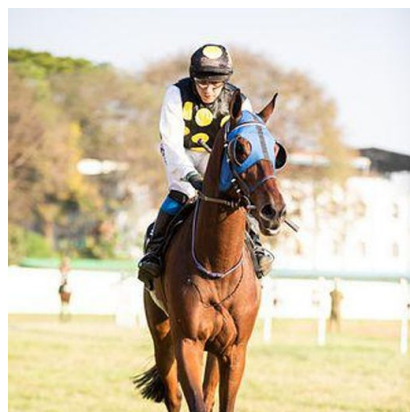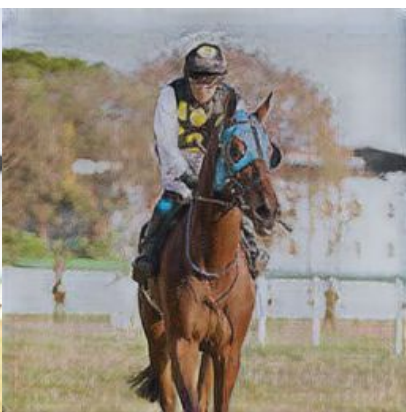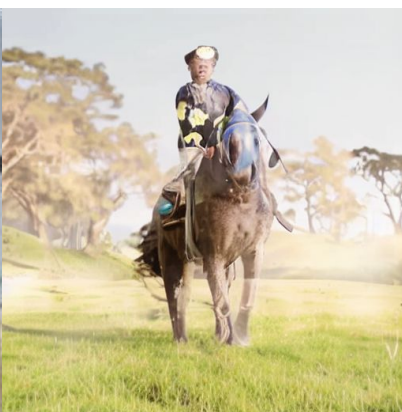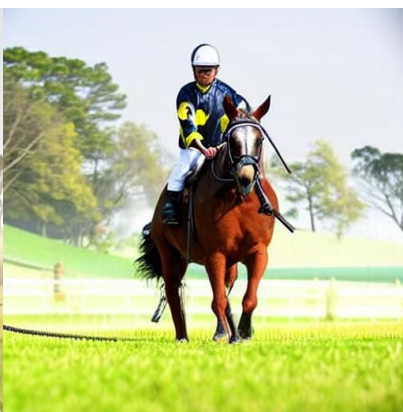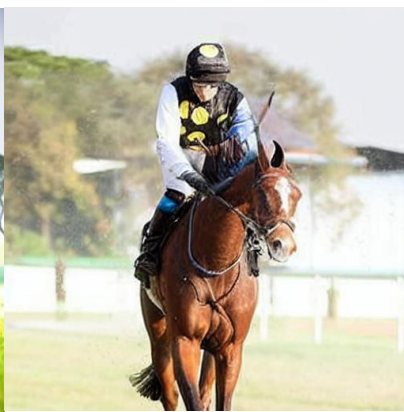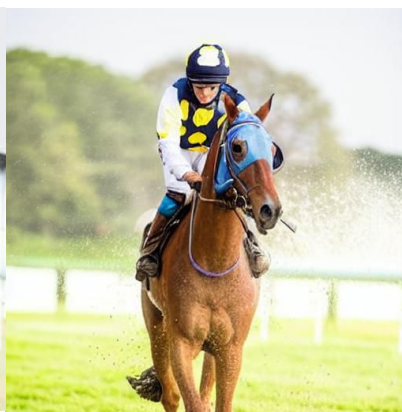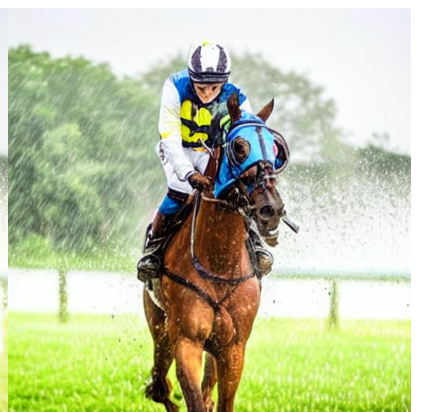

Prompt: 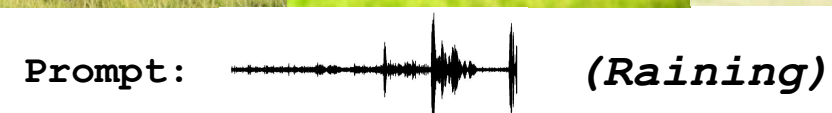 (*Raining*)
