# Supplementary material for: Audio-Guided Visual Editing with Complex Multi-Modal Prompts
Source: arXiv:2508.20379 source file (2025-08-28)
Supplement: Supplementary file 3 [file figure_A2V_supp.pdf]

Original

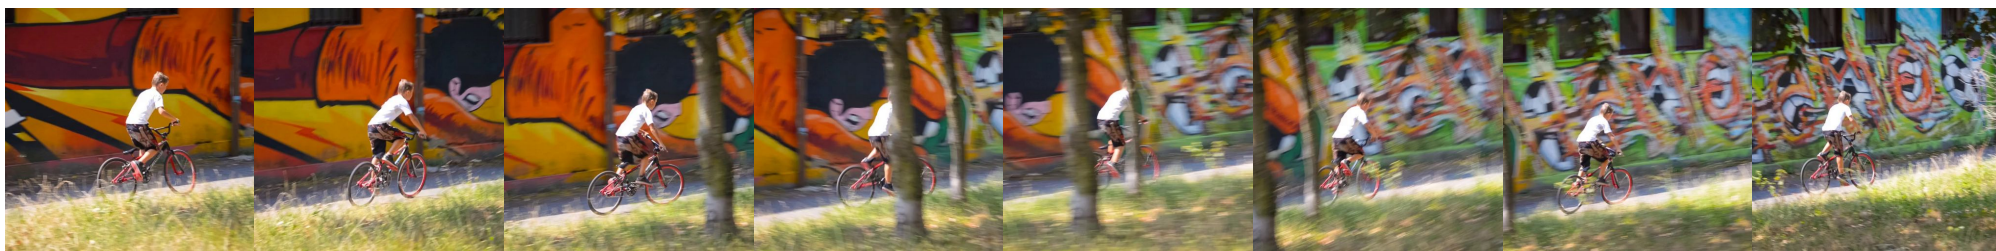

Tokenflow

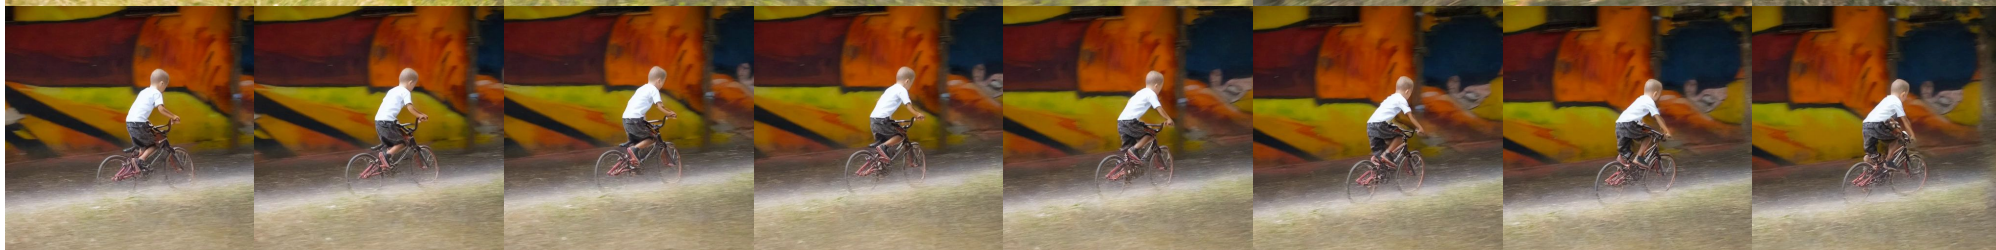

Gen1

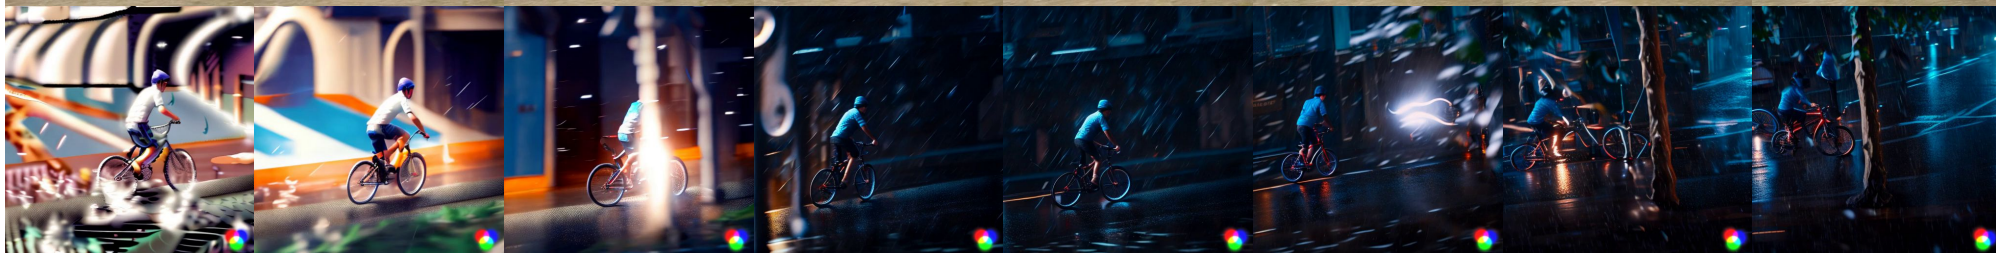

Ours

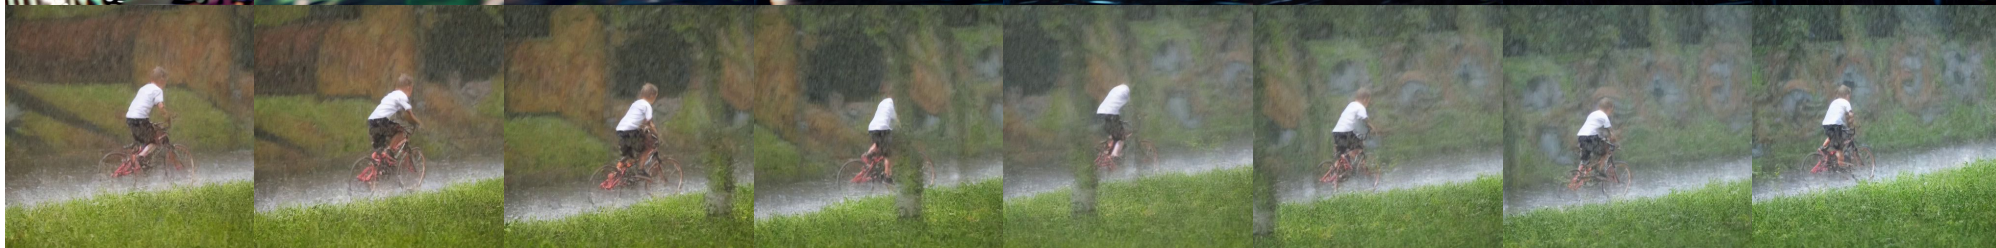

Prompt: 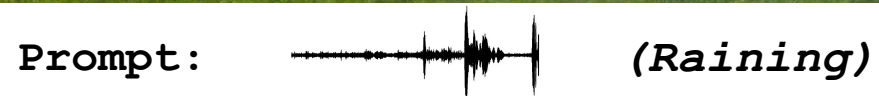 (Raining)

Original

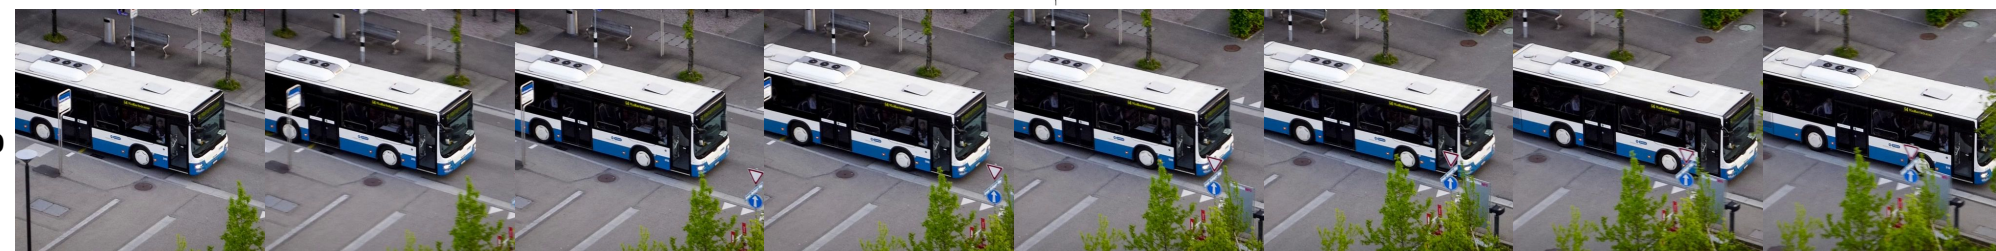

Tokenflow

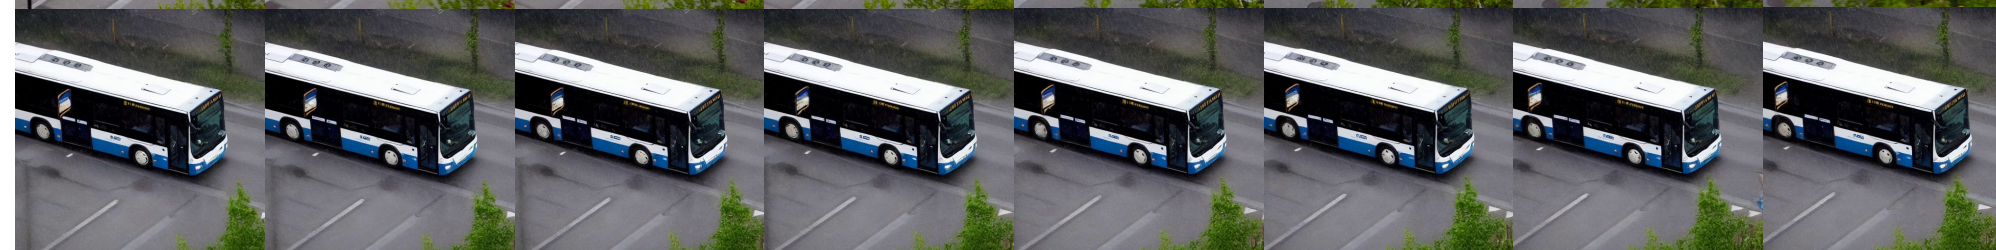

Gen1

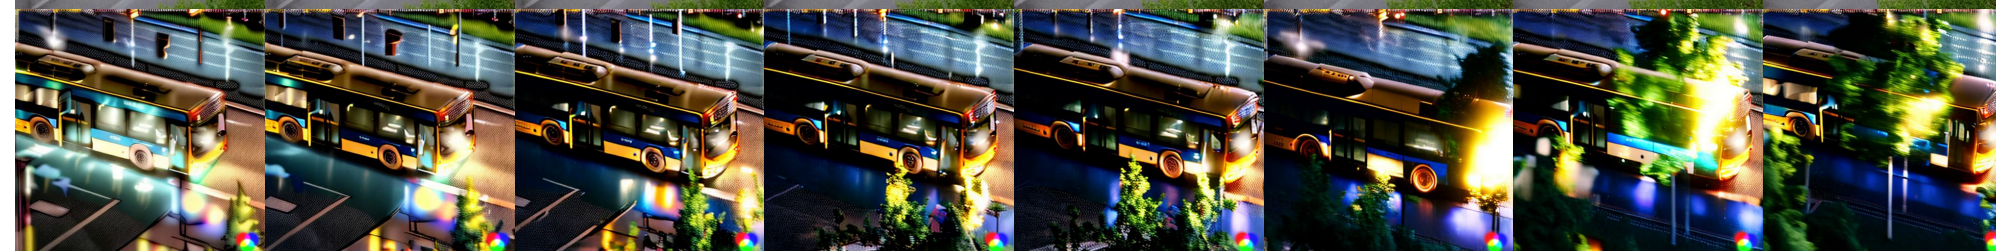

Ours

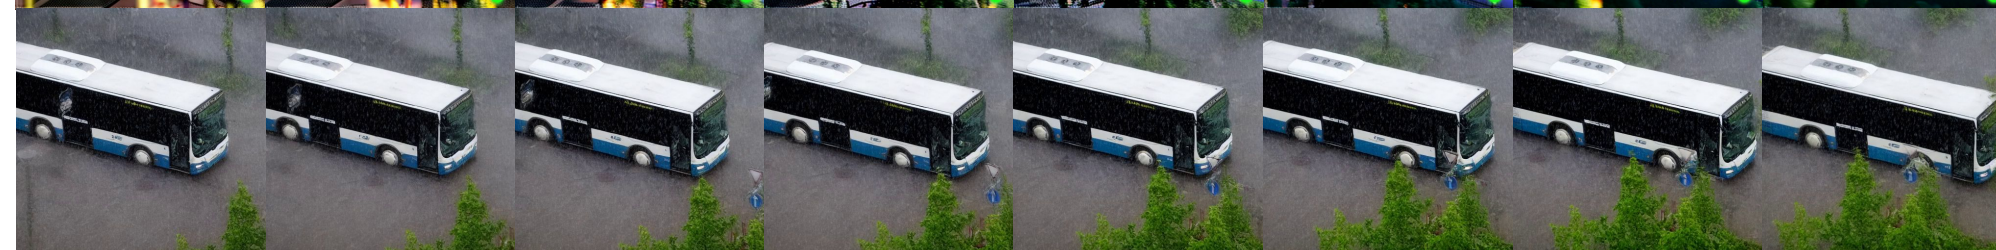

Prompt: 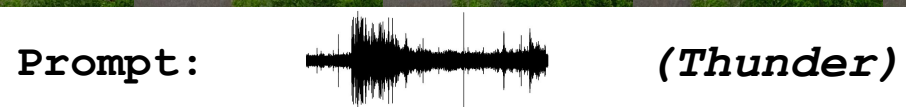 (Thunder)



Original

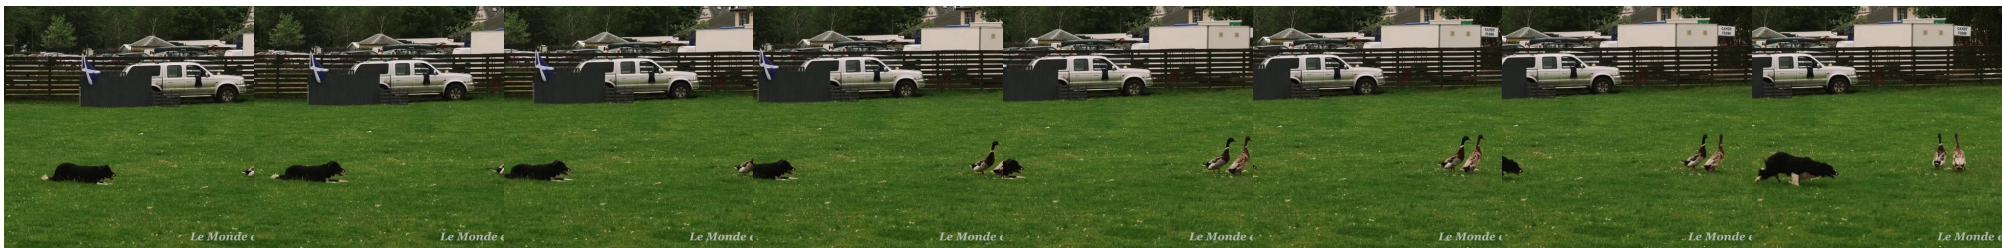

Tokenflow

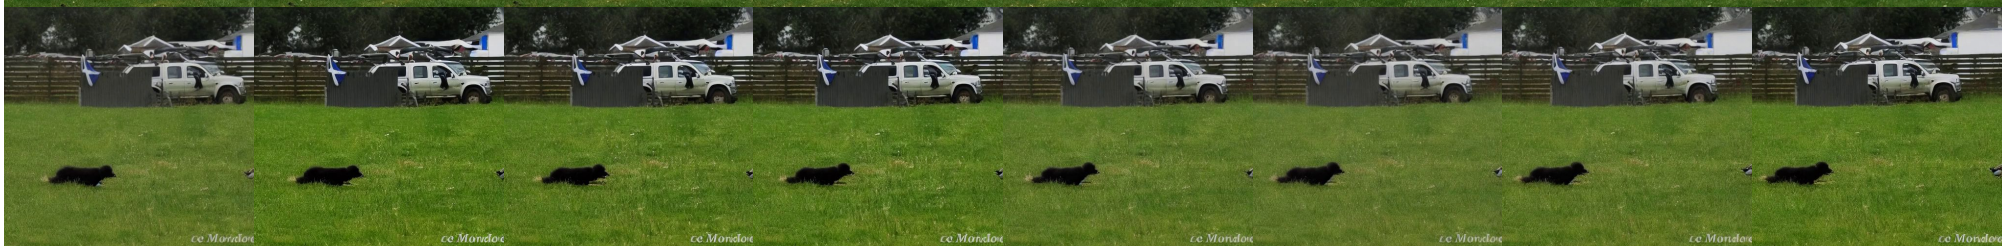

Gen1

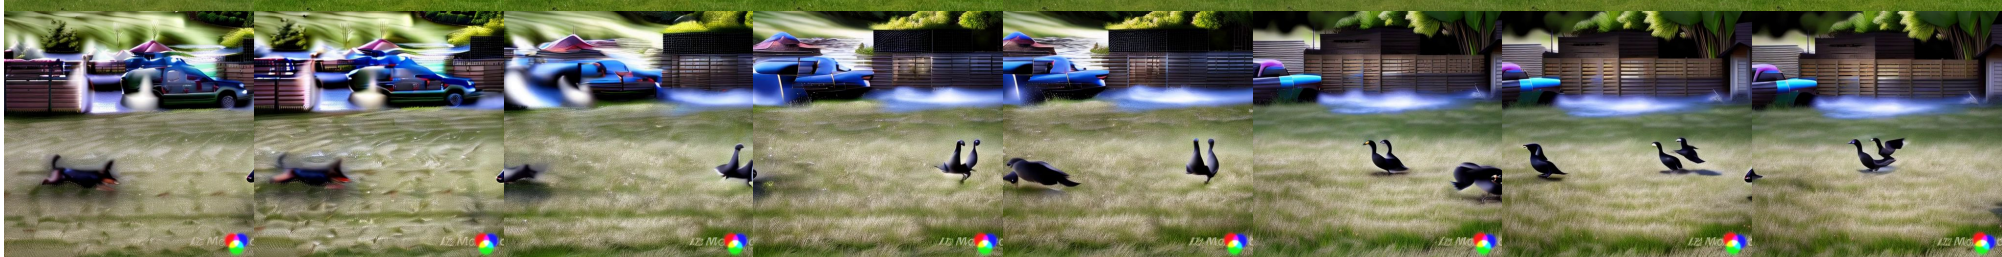

Ours

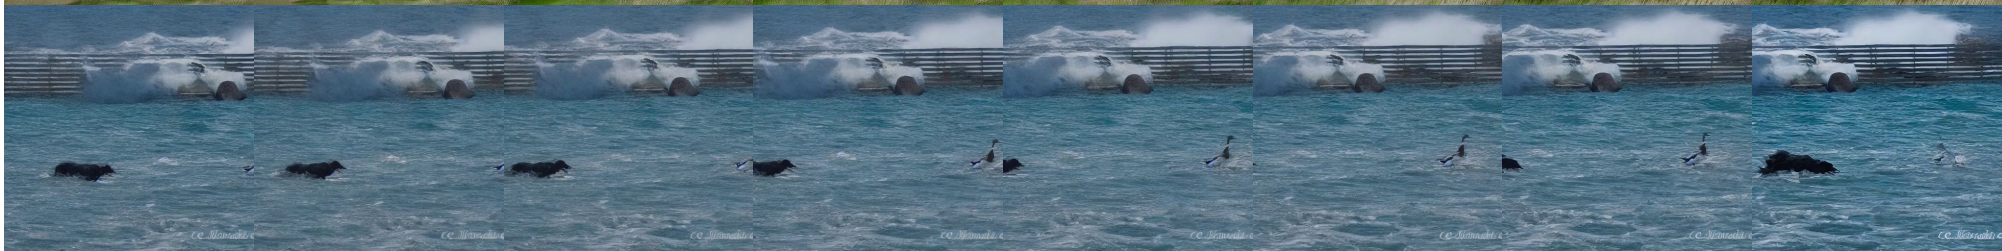

Prompt:

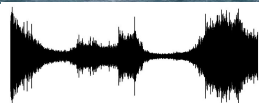

(Sea Waves)

Original

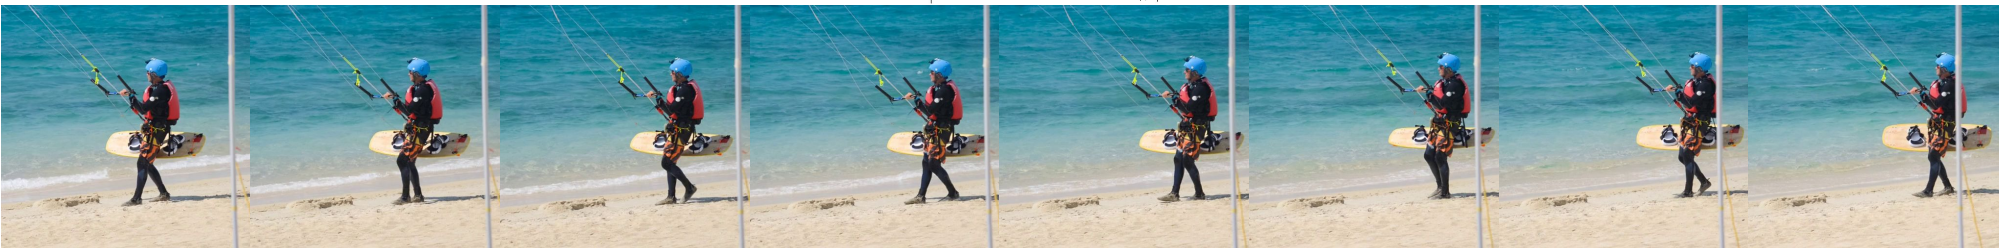

Tokenflow

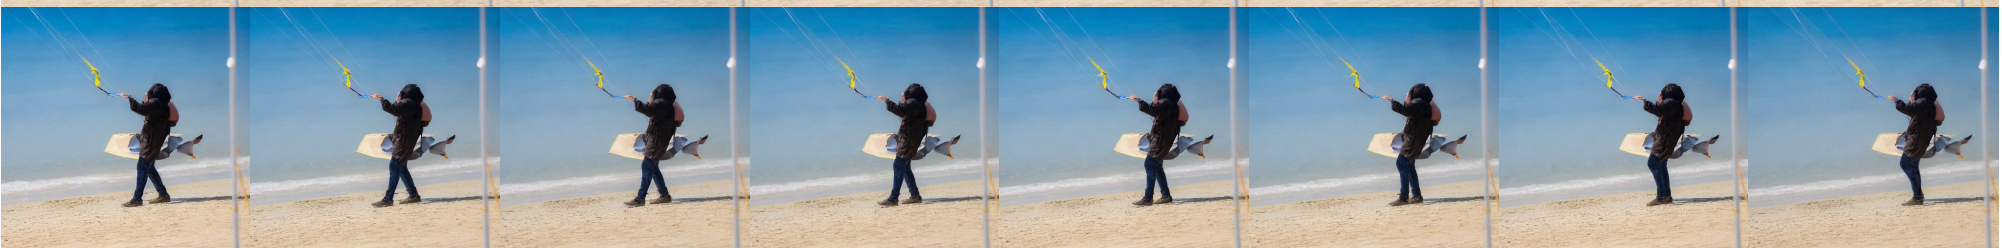

Gen1

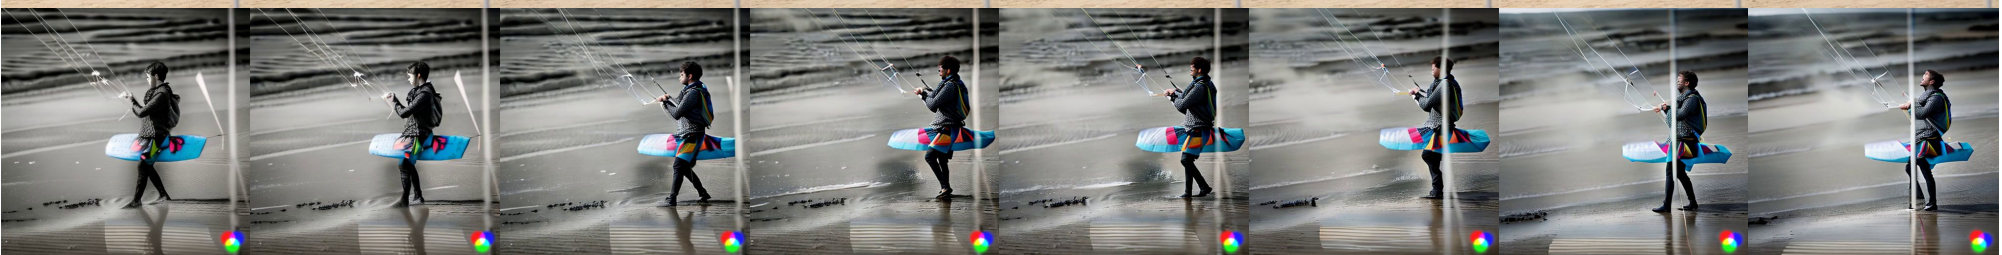

Ours

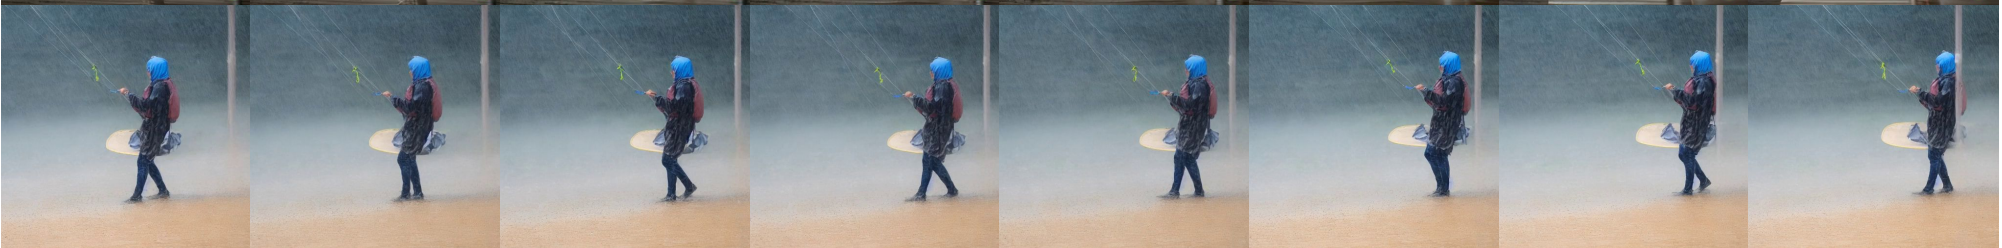

Prompt:

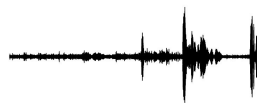

(Raining)
