# Supplementary material for: Audio-Guided Visual Editing with Complex Multi-Modal Prompts
Source: arXiv:2508.20379 source file (2025-08-28)
Supplement: Supplementary file 4 [file figure_multiple_supp.pdf]

## Source image

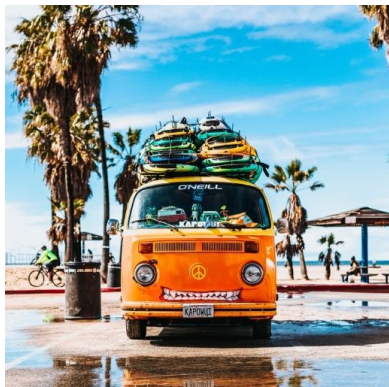

## Prompt #1

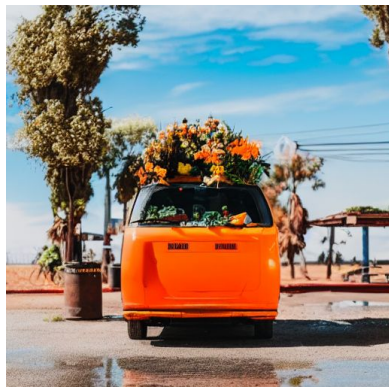

An orange van  
with **surfboards**  
**flowers** on top

## Prompt #2

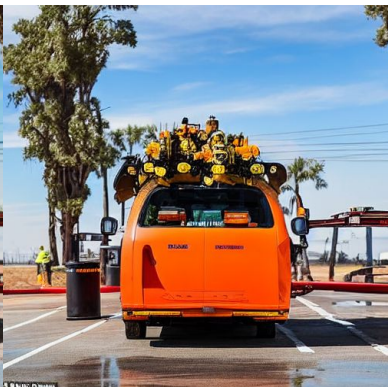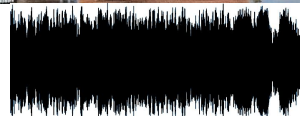

(Fire Truck  
Siren)

## Prompt #3

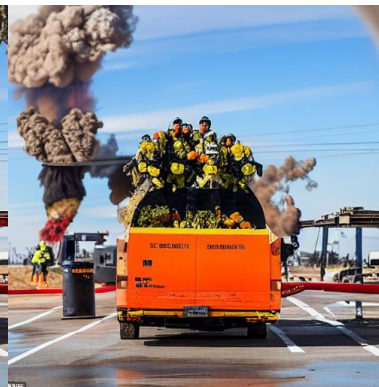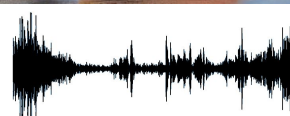

(Volcano  
Explosion)

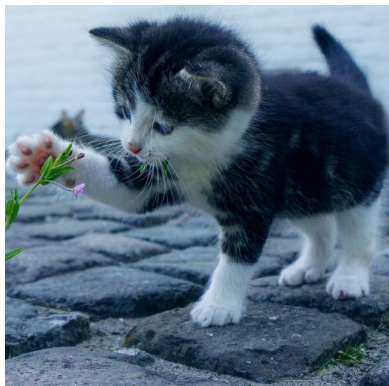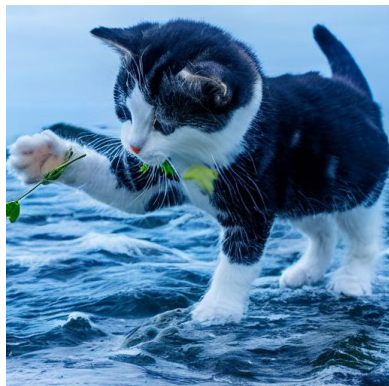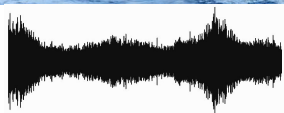

(Sea Waves)

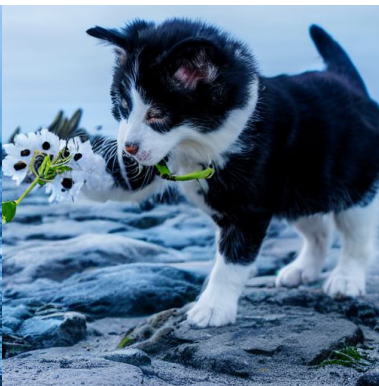

Blue light, a  
black and white  
**cat dog** is playing  
with a flower

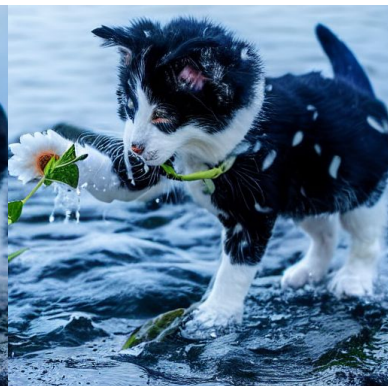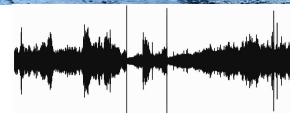

(Splashing  
Water)

Source image

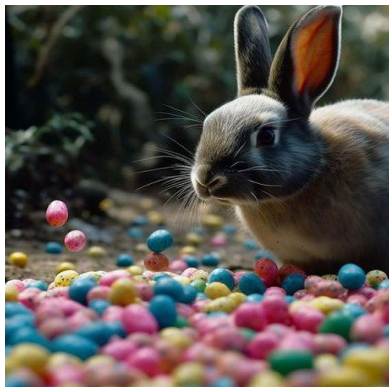

Prompt #1

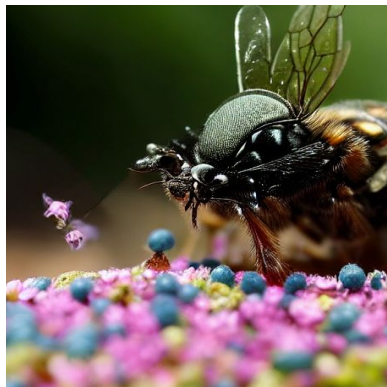

*(Bee, Wasp,  
etc. Buzzing)*

Prompt #2

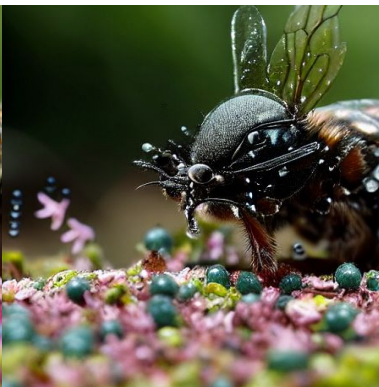

*(Raining)*

Prompt #3

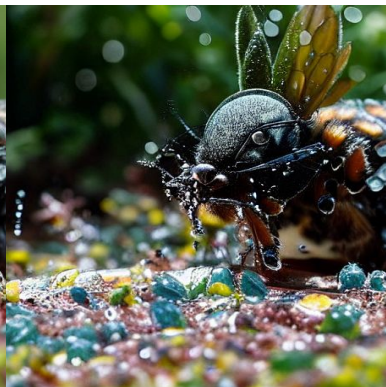

*(Splashing  
Water)*

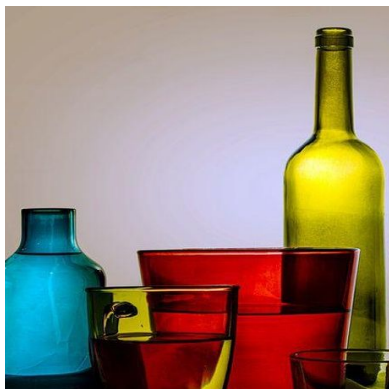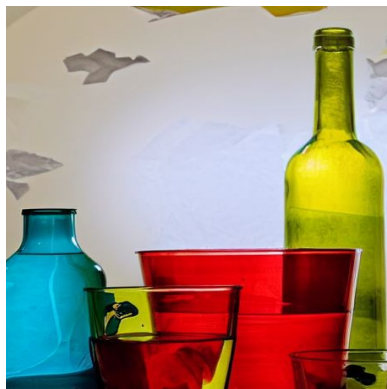

*(Ripping Paper)*

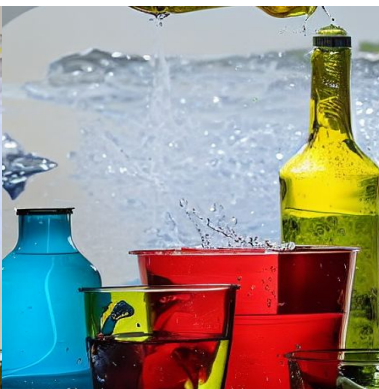

*(Splashing Water)*

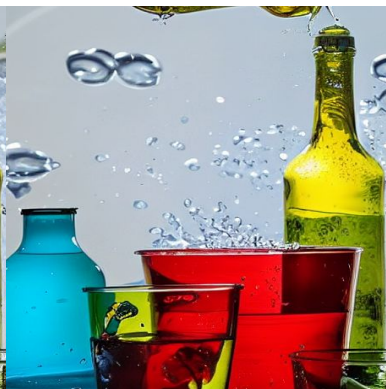

*(Underwater  
Bubbling)*
